# Supplementary material for: Metaplectic geometrical optics for modeling caustics in uniform and nonuniform media
Source: arXiv:2009.03220 ancillary file (2021-03-08)
Supplement: Supplementary file 1 [file supplement.pdf]

# Supplementary material for "Metaplectic geometrical optics for modeling caustics in uniform and nonuniform media"

N. A. Lopez[1] and I. Y. Dodin[1,2]

[1]*Department of Astrophysical Sciences, Princeton University, Princeton, New Jersey 08544, USA*
[2]*Princeton Plasma Physics Laboratory, Princeton, New Jersey 08543, USA*

This supplementary document provides complete derivations for Secs. 3 and 4 of the main text.

## I. METAPLECTIC GEOMETRICAL OPTICS WITH COHERENT STATES

### A. Introduction

A coherent state centered on $\mathbf{z}_0 = (\mathbf{q}_0, \mathbf{p}_0)$ in phase space is defined as a state $|\mathbf{z}_0\rangle$ whose coordinate representation is [1, Eq. (C.8), p. 287]

$$\langle \mathbf{q}|\mathbf{z}_0\rangle = \pi^{-N/4} \exp\left[-\frac{1}{2}(\mathbf{q}-\mathbf{q}_0)^\intercal(\mathbf{q}-\mathbf{q}_0) + i\mathbf{p}_0^\intercal\mathbf{q} - \frac{i}{2}\mathbf{p}_0^\intercal\mathbf{q}_0\right] , \tag{S1}$$

or equivalently [1, Eq. (C.9), p. 287],

$$\langle \mathbf{q}|\mathbf{z}_0\rangle = \pi^{-N/4} \exp\left[-\frac{1}{2}\mathbf{q}^\intercal\mathbf{q} + \mathbf{q}^\intercal\boldsymbol{\zeta} - \frac{1}{4}(\boldsymbol{\zeta}+\boldsymbol{\zeta}^*)^\intercal\boldsymbol{\zeta}\right] , \tag{S2}$$

where we have introduced the $N$-D complex vectors

$$\boldsymbol{\zeta} \doteq \mathbf{q}_0 + i\mathbf{p}_0 , \quad \boldsymbol{\zeta}^* \doteq \mathbf{q}_0 - i\mathbf{p}_0 . \tag{S3}$$

Such states have a unit norm ($\langle \mathbf{z}_0|\mathbf{z}_0\rangle = 1$), form a complete basis in the Hilbert space of functions on $\mathbf{q}$-space, and satisfy [1, Eq. (C.2), p. 286] [1]

$$\hat{\mathbb{1}} = \int \frac{\mathrm{d}\mathbf{q}_0\mathrm{d}\mathbf{p}_0}{(2\pi)^N} |\mathbf{z}_0\rangle\langle\mathbf{z}_0| . \tag{S4}$$

In particular, this means

$$\langle \mathbf{q}|\mathbf{Q}(\mathbf{q}')\rangle = \langle \mathbf{q}|\hat{M}^\dagger|\mathbf{q}'\rangle = \int \frac{\mathrm{d}\mathbf{q}_0\mathrm{d}\mathbf{p}_0}{(2\pi)^N} \langle \mathbf{q}|\hat{M}^\dagger|\mathbf{z}_0\rangle\langle\mathbf{z}_0|\mathbf{q}'\rangle . \tag{S5}$$

Then, the metaplectic transform (MT) can be written as

$$\psi(\mathbf{q}) = \int \mathrm{d}\mathbf{q}' \, \langle \mathbf{q}|\mathbf{Q}(\mathbf{q}')\rangle\langle\mathbf{Q}(\mathbf{q}')|\psi\rangle = \int \frac{\mathrm{d}\mathbf{q}_0\mathrm{d}\mathbf{p}_0\mathrm{d}\mathbf{q}'}{(2\pi)^N} \langle \mathbf{q}|\hat{M}^\dagger|\mathbf{z}_0\rangle \, \langle\mathbf{z}_0|\mathbf{q}'\rangle \, \Psi(\mathbf{q}') , \tag{S6}$$

where $\langle\mathbf{z}_0|\mathbf{q}'\rangle$ is just a Gaussian. Below, we show how to calculate $\langle \mathbf{q}|\hat{M}^\dagger|\mathbf{z}_0\rangle$ and how to calculate the saddlepoints of the integral (S6). For completeness, we also derive some basic properties of coherent states in the appendix in the end of this section.

### B. Calculation of the MT matrix element

Let us consider

$$\begin{aligned}\langle \mathbf{q}|\hat{M}|\mathbf{z}_0\rangle &= \int \mathrm{d}\mathbf{q}' \, \langle \mathbf{q}|\hat{M}|\mathbf{q}'\rangle \, \langle\mathbf{q}'|\mathbf{z}_0\rangle \\ &= \frac{1}{\pi^{N/4}} \int \mathrm{d}\mathbf{q}' \, \langle \mathbf{q}|\hat{M}|\mathbf{q}'\rangle \, \exp\left[-\frac{1}{2}(\mathbf{q}')^\intercal\mathbf{q}' + (\mathbf{q}')^\intercal\boldsymbol{\zeta} - \frac{1}{4}(\boldsymbol{\zeta}+\boldsymbol{\zeta}^*)^\intercal\boldsymbol{\zeta}\right] ,\end{aligned} \tag{S7}$$

---

[1] It is interesting to note that this completeness relation does not depend on Eq. (S1) per se, but rather it is a property of the phase-space translation operators $\hat{T}(\mathbf{z}_0) \doteq \exp\left(-i\mathbf{z}_0^\intercal\mathsf{J}\hat{\mathbf{z}}\right)$. Any normalized and sufficiently localized state can be used to construct a family of 'coherent states' via $\hat{T}(\mathbf{z}_0)$ that satisfy a completeness relation analogous to Eq. (S4).

and a matrix

$$\mathsf{S} \doteq \begin{pmatrix} \mathsf{A} & \mathsf{B} \\ \mathsf{C} & \mathsf{D} \end{pmatrix} \tag{S8}$$

that is symplectic [Eq. (15) of the main text]. For simplicity, let us assume $\det \mathsf{B} \neq 0$. (The case $\det \mathsf{B} = 0$ will be considered later as a limit.) Then, we can use Eq. (17) of the main text to express $\langle \mathbf{q}|\hat{M}|\mathbf{q}'\rangle$ as follows:

$$\langle \mathbf{q}|\hat{M}|\mathbf{q}'\rangle = \frac{\sigma}{(2\pi i)^{N/2}\sqrt{\det \mathsf{B}}} \exp\left[\frac{i}{2}\mathbf{q}^\intercal \mathsf{D}\mathsf{B}^{-1}\mathbf{q} - i(\mathbf{q}')^\intercal \mathsf{B}^{-1}\mathbf{q} + \frac{i}{2}(\mathbf{q}')^\intercal \mathsf{B}^{-1}\mathsf{A}\mathbf{q}'\right]. \tag{S9}$$

Then,

$$\begin{aligned}
\langle \mathbf{q}|\hat{M}|\mathbf{q}'\rangle \langle \mathbf{q}'|\mathbf{z}_0\rangle &= \frac{\sigma}{\pi^{N/4}(2\pi i)^{N/2}\sqrt{\det \mathsf{B}}} \exp\left[\frac{i}{2}\mathbf{q}^\intercal \mathsf{D}\mathsf{B}^{-1}\mathbf{q} - i(\mathbf{q}')^\intercal \mathsf{B}^{-1}\mathbf{q} + \frac{i}{2}(\mathbf{q}')^\intercal \mathsf{B}^{-1}\mathsf{A}\mathbf{q}' \right. \\
&\qquad \left. -\frac{1}{2}(\mathbf{q}')^\intercal \mathbf{q}' + (\mathbf{q}')^\intercal \boldsymbol{\zeta} - \frac{1}{4}(\boldsymbol{\zeta} + \boldsymbol{\zeta}^*)^\intercal \boldsymbol{\zeta}\right] \\
&= \frac{\sigma \exp\left[\frac{i}{2}\mathbf{q}^\intercal \mathsf{D}\mathsf{B}^{-1}\mathbf{q} - \frac{1}{4}(\boldsymbol{\zeta} + \boldsymbol{\zeta}^*)^\intercal \boldsymbol{\zeta}\right]}{\pi^{N/4}(2\pi i)^{N/2}\sqrt{\det \mathsf{B}}} \exp\left[\frac{i}{2}(\mathbf{q}')^\intercal \mathsf{B}^{-1}\left(\mathsf{A} + i\mathsf{B}\right)\mathbf{q}' + i(\mathbf{q}')^\intercal\left(-i\boldsymbol{\zeta} - \mathsf{B}^{-1}\mathbf{q}\right)\right].
\end{aligned} \tag{S10}$$

Thus, using

$$\int \mathrm{d}\mathbf{x}\, \exp\left(\frac{i}{2}\mathbf{x}^\intercal \mathsf{M}\mathbf{x} + i\mathbf{x}^\intercal \mathbf{v}\right) = \frac{(2\pi i)^{N/2}}{\sqrt{\det \mathsf{M}}}\, \exp\left(-\frac{i}{2}\mathbf{v}^\intercal \mathsf{M}^{-1}\mathbf{v}\right) \tag{S11}$$

(depending on the branch of the square root, an overall minus sign may need to be added but will be absorbed in $\sigma$), we compute

$$\begin{aligned}
\langle \mathbf{q}|\hat{M}|\mathbf{z}_0\rangle &= \frac{\sigma \exp\left[\frac{i}{2}\mathbf{q}^\intercal \mathsf{D}\mathsf{B}^{-1}\mathbf{q} - \frac{1}{4}(\boldsymbol{\zeta} + \boldsymbol{\zeta}^*)^\intercal \boldsymbol{\zeta}\right]}{\pi^{N/4}(2\pi i)^{N/2}\sqrt{\det \mathsf{B}}} \int \mathrm{d}\mathbf{q}'\, \exp\left[\frac{i}{2}(\mathbf{q}')^\intercal \mathsf{B}^{-1}\left(\mathsf{A} + i\mathsf{B}\right)\mathbf{q}' + i(\mathbf{q}')^\intercal\left(-i\boldsymbol{\zeta} - \mathsf{B}^{-1}\mathbf{q}\right)\right] \\
&= \frac{\sigma \exp\left[\frac{i}{2}\mathbf{q}^\intercal \mathsf{D}\mathsf{B}^{-1}\mathbf{q} - \frac{1}{4}(\boldsymbol{\zeta} + \boldsymbol{\zeta}^*)^\intercal \boldsymbol{\zeta}\right]}{\pi^{N/4}(2\pi i)^{N/2}\sqrt{\det \mathsf{B}}} \\
&\quad \times \frac{(2\pi i)^{N/2}\sqrt{\det \mathsf{B}}}{\sqrt{\det(\mathsf{A} + i\mathsf{B})}} \exp\left[-\frac{i}{2}\left(-i\boldsymbol{\zeta} - \mathsf{B}^{-1}\mathbf{q}\right)^\intercal \left(\mathsf{A} + i\mathsf{B}\right)^{-1}\mathsf{B}\left(-i\boldsymbol{\zeta} - \mathsf{B}^{-1}\mathbf{q}\right)\right] \\
&= \frac{\sigma}{\pi^{N/4}\sqrt{\det(\mathsf{A} + i\mathsf{B})}} \exp\left\{-\frac{1}{2}\mathbf{q}^\intercal\left[i\mathsf{B}^{-\intercal} - i\mathsf{D}\mathsf{B}^{-1}\left(\mathsf{A} + i\mathsf{B}\right)\right]\left(\mathsf{A} + i\mathsf{B}\right)^{-1}\mathbf{q} \right. \\
&\qquad \left. +\boldsymbol{\zeta}^\intercal\left(\mathsf{A} + i\mathsf{B}\right)^{-1}\mathbf{q} - \frac{1}{4}(\boldsymbol{\zeta} + \boldsymbol{\zeta}^*)^\intercal \boldsymbol{\zeta} + \frac{i}{2}\boldsymbol{\zeta}^\intercal\left(\mathsf{A} + i\mathsf{B}\right)^{-1}\mathsf{B}\boldsymbol{\zeta}\right\}.
\end{aligned} \tag{S12}$$

Using Eqs. (A1a) and (A1c) of the main text, we simplify

$$i\mathsf{B}^{-\intercal} - i\mathsf{D}\mathsf{B}^{-1}\left(\mathsf{A} + i\mathsf{B}\right) = i\mathsf{B}^{-\intercal} - i\mathsf{D}\mathsf{B}^{-1}\mathsf{A} + \mathsf{D} = \mathsf{D} - i\mathsf{C}. \tag{S13}$$

Thus, we obtain

$$\begin{aligned}
\langle \mathbf{q}|\hat{M}|\mathbf{z}_0\rangle &= \frac{\sigma}{\pi^{N/4}\sqrt{\det(\mathsf{A} + i\mathsf{B})}} \\
&\quad \times \exp\left[-\frac{1}{2}\mathbf{q}^\intercal\left(\mathsf{D} - i\mathsf{C}\right)\left(\mathsf{A} + i\mathsf{B}\right)^{-1}\mathbf{q} + \boldsymbol{\zeta}^\intercal\left(\mathsf{A} + i\mathsf{B}\right)^{-1}\mathbf{q} - \frac{1}{4}(\boldsymbol{\zeta} + \boldsymbol{\zeta}^*)^\intercal \boldsymbol{\zeta} + \frac{i}{2}\boldsymbol{\zeta}^\intercal\left(\mathsf{A} + i\mathsf{B}\right)^{-1}\mathsf{B}\boldsymbol{\zeta}\right],
\end{aligned} \tag{S14}$$

in agreement with Eq. (6.32) of Ref. [1, p. 248]. Importantly, both $(\mathsf{D} - i\mathsf{C})(\mathsf{A} + i\mathsf{B})^{-1}$ and $\left(\mathsf{A} + i\mathsf{B}\right)^{-1}\mathsf{B}$ are symmetric because

$$(\mathsf{D} - i\mathsf{C})(\mathsf{A} + i\mathsf{B})^{-1} = (\mathsf{A} + i\mathsf{B})^{-\intercal}\left[\mathsf{I}_N + \mathsf{C}^\intercal\mathsf{B} + \mathsf{B}^\intercal\mathsf{C} + i(\mathsf{B}^\intercal\mathsf{D} - \mathsf{A}^\intercal\mathsf{C})\right](\mathsf{A} + i\mathsf{B})^{-1}, \tag{S15a}$$

$$\left(\mathsf{A} + i\mathsf{B}\right)^{-1}\mathsf{B} = \left(\mathsf{A} + i\mathsf{B}\right)^{-1}\left(\mathsf{B}\mathsf{A}^\intercal + i\mathsf{B}\mathsf{B}^\intercal\right)\left(\mathsf{A} + i\mathsf{B}\right)^{-\intercal}, \tag{S15b}$$

where the matrices on the right-hand side are symmetric by Eqs. (A1a), (A1b), and (A1e) from the main text.

Although we assumed $\det \mathsf{B} \neq 0$, the final result (S14) holds even when $\det \mathsf{B} = 0$, so we can consider it as the analytic continuation to all values of $\det \mathsf{B}$. Also, note that $\det(\mathsf{A} + i\mathsf{B}) \neq 0$ by symplecticity of $\mathsf{S}$ [1, 2]. Thus, using

$$\hat{M}^\dagger(\mathsf{S}) = \pm \hat{M}(\mathsf{S}^{-1}) \, , \quad \mathsf{S}^{-1} = \begin{pmatrix} \mathsf{D}^\intercal & -\mathsf{B}^\intercal \\ -\mathsf{C}^\intercal & \mathsf{A}^\intercal \end{pmatrix} \, , \tag{S16}$$

we obtain

$$\langle \mathbf{q} | \hat{M}^\dagger | \mathbf{z}_0 \rangle = \frac{\sigma}{\pi^{N/4} \sqrt{\det(\mathsf{D} - i\mathsf{B})}} \times \exp\left[ -\frac{1}{2} \mathbf{q}^\intercal \left(\mathsf{D} - i\mathsf{B}\right)^{-1} \left(\mathsf{A} + i\mathsf{C}\right) \mathbf{q} + \mathbf{q}^\intercal \left(\mathsf{D} - i\mathsf{B}\right)^{-1} \boldsymbol{\zeta} - \frac{1}{4} (\boldsymbol{\zeta} + \boldsymbol{\zeta}^*)^\intercal \boldsymbol{\zeta} - \frac{i}{2} \boldsymbol{\zeta}^\intercal \mathsf{B} \left(\mathsf{D} - i\mathsf{B}\right)^{-1} \boldsymbol{\zeta} \right] \, , \tag{S17}$$

where we have also used the fact that $\left(\mathsf{D} - i\mathsf{B}\right)^{-1} \left(\mathsf{A} + i\mathsf{C}\right)$ and $\mathsf{B} \left(\mathsf{D} - i\mathsf{B}\right)^{-1}$ are both symmetric, for reasons analogous to Eqs. (S15). Again, note that $\det(\mathsf{D} - i\mathsf{B}) \neq 0$ always [1, 2].

Using Eq. (S17), we compute

$$\begin{aligned}
\langle \mathbf{q} | \hat{M}^\dagger | \mathbf{z}_0 \rangle \langle \mathbf{z}_0 | \mathbf{q}' \rangle &= \frac{\sigma}{\pi^{N/4} \sqrt{\det(\mathsf{D} - i\mathsf{B})}} \\
&\quad \times \exp\left[ -\frac{1}{2} \mathbf{q}^\intercal \left(\mathsf{D} - i\mathsf{B}\right)^{-1} \left(\mathsf{A} + i\mathsf{C}\right) \mathbf{q} + \mathbf{q}^\intercal \left(\mathsf{D} - i\mathsf{B}\right)^{-1} \boldsymbol{\zeta} - \frac{1}{4} (\boldsymbol{\zeta} + \boldsymbol{\zeta}^*)^\intercal \boldsymbol{\zeta} - \frac{i}{2} \boldsymbol{\zeta}^\intercal \mathsf{B} \left(\mathsf{D} - i\mathsf{B}\right)^{-1} \boldsymbol{\zeta} \right] \\
&\quad \times \pi^{-N/4} \exp\left[ -\frac{1}{2} (\mathbf{q}')^\intercal \mathbf{q}' + (\mathbf{q}')^\intercal \boldsymbol{\zeta}^* - \frac{1}{4} (\boldsymbol{\zeta} + \boldsymbol{\zeta}^*)^\intercal \boldsymbol{\zeta}^* \right] \\
&= \frac{\sigma \, \exp\left[ -\frac{1}{2} \mathbf{q}^\intercal \left(\mathsf{D} - i\mathsf{B}\right)^{-1} \left(\mathsf{A} + i\mathsf{C}\right) \mathbf{q} \right]}{\pi^{N/2} \sqrt{\det(\mathsf{D} - i\mathsf{B})}} \\
&\quad \times \exp\left[ -\frac{1}{2} (\mathbf{q}')^\intercal \mathbf{q}' + (\mathbf{q}')^\intercal \boldsymbol{\zeta}^* + \mathbf{q}^\intercal \left(\mathsf{D} - i\mathsf{B}\right)^{-1} \boldsymbol{\zeta} - \frac{i}{2} \boldsymbol{\zeta}^\intercal \mathsf{B} \left(\mathsf{D} - i\mathsf{B}\right)^{-1} \boldsymbol{\zeta} - \frac{1}{4} (\boldsymbol{\zeta} + \boldsymbol{\zeta}^*)^\intercal (\boldsymbol{\zeta} + \boldsymbol{\zeta}^*) \right] .
\end{aligned} \tag{S18}$$

Hence, Eq. (S6) becomes

$$\psi(\mathbf{q}) = \frac{\sigma \exp\left[ -\frac{1}{2} \mathbf{q}^\intercal \left(\mathsf{D} - i\mathsf{B}\right)^{-1} \left(\mathsf{A} + i\mathsf{C}\right) \mathbf{q} \right]}{(2\pi)^N \pi^{N/2} \sqrt{\det(\mathsf{D} - i\mathsf{B})}} \times \int \mathrm{d}\mathbf{Q} \, \mathrm{d}\mathbf{q}_0 \, \mathrm{d}\mathbf{p}_0 \, \Psi(\mathbf{Q}) \exp\left[ -\frac{1}{2} \mathbf{Q}^\intercal \mathbf{Q} - \frac{i}{2} \boldsymbol{\zeta}^\intercal \mathsf{B} \left(\mathsf{D} - i\mathsf{B}\right)^{-1} \boldsymbol{\zeta} - \mathbf{q}_0^\intercal \mathbf{q}_0 + \mathbf{Q}^\intercal \boldsymbol{\zeta}^* + \mathbf{q}^\intercal \left(\mathsf{D} - i\mathsf{B}\right)^{-1} \boldsymbol{\zeta} \right] \, , \tag{S19}$$

where we have replaced the dummy variable $\mathbf{q}'$ with $\mathbf{Q}$. The MT can also be written as

$$\begin{aligned}
\psi(\mathbf{q}) &= \frac{\sigma \exp\left[ -\frac{1}{2} \mathbf{q}^\intercal \left(\mathsf{D} - i\mathsf{B}\right)^{-1} \left(\mathsf{A} + i\mathsf{C}\right) \mathbf{q} \right]}{(2\pi)^N \pi^{N/2} \sqrt{\det(\mathsf{D} - i\mathsf{B})}} \\
&\quad \times \int \mathrm{d}\mathbf{Q} \, \mathrm{d}\mathbf{p}_0 \, \mathrm{d}\mathbf{q}_0 \, \Psi(\mathbf{Q}) \exp\left\{ -\frac{1}{2} \mathbf{Q}^\intercal \mathbf{Q} + \frac{i}{2} \mathbf{p}_0^\intercal \mathsf{B} \left(\mathsf{D} - i\mathsf{B}\right)^{-1} \mathbf{p}_0 + i \mathbf{p}_0^\intercal \left[ \left(\mathsf{D} - i\mathsf{B}\right)^{-\intercal} \mathbf{q} - \mathbf{Q} \right] \right. \\
&\qquad \left. - \frac{1}{2} \mathbf{q}_0^\intercal \left(2\mathsf{D} - i\mathsf{B}\right) \left(\mathsf{D} - i\mathsf{B}\right)^{-1} \mathbf{q}_0 + \mathbf{q}_0^\intercal \left[ \left(\mathsf{D} - i\mathsf{B}\right)^{-\intercal} \mathbf{q} + \mathbf{Q} + \mathsf{B} \left(\mathsf{D} - i\mathsf{B}\right)^{-1} \mathbf{p}_0 \right] \right\} ,
\end{aligned} \tag{S20}$$

or equivalently,

$$\begin{aligned}
\psi(\mathbf{q}) &= \frac{\sigma \exp\left[ -\frac{1}{2} \mathbf{q}^\intercal \left(\mathsf{D} - i\mathsf{B}\right)^{-1} \left(\mathsf{A} + i\mathsf{C}\right) \mathbf{q} \right]}{(2\pi)^N \pi^{N/2} \sqrt{\det(\mathsf{D} - i\mathsf{B})}} \\
&\quad \times \int \mathrm{d}\mathbf{Q} \, \mathrm{d}\mathbf{q}_0 \, \mathrm{d}\mathbf{p}_0 \, \Psi(\mathbf{Q}) \exp\left\{ -\frac{1}{2} \mathbf{Q}^\intercal \mathbf{Q} - \frac{1}{2} \mathbf{q}_0^\intercal \left(2\mathsf{D} - i\mathsf{B}\right) \left(\mathsf{D} - i\mathsf{B}\right)^{-1} \mathbf{q}_0 + \mathbf{q}_0^\intercal \left[ \left(\mathsf{D} - i\mathsf{B}\right)^{-\intercal} \mathbf{q} + \mathbf{Q} \right] \right. \\
&\qquad \left. + \frac{i}{2} \mathbf{p}_0^\intercal \mathsf{B} \left(\mathsf{D} - i\mathsf{B}\right)^{-1} \mathbf{p}_0 + i \mathbf{p}_0^\intercal \left[ \left(\mathsf{D} - i\mathsf{B}\right)^{-\intercal} \mathbf{q} - \mathbf{Q} - i\mathsf{B} \left(\mathsf{D} - i\mathsf{B}\right)^{-1} \mathbf{q}_0 \right] \right\} .
\end{aligned} \tag{S21}$$

Indeed, we can recover the original inverse MT [Eq. (35) in the main text] by performing the integration over $\mathbf{p}_0$ in Eq. (S21) as

$$\begin{aligned}
&\int \mathrm{d}\mathbf{p}_0 \, \exp\left\{ \frac{i}{2}\mathbf{p}_0^\intercal \mathsf{B} \left(\mathsf{D} - i\mathsf{B}\right)^{-1} \mathbf{p}_0 + i\mathbf{p}_0^\intercal \left[ \left(\mathsf{D} - i\mathsf{B}\right)^{-\intercal} \mathbf{q} - \mathbf{Q} - i\mathsf{B}\left(\mathsf{D} - i\mathsf{B}\right)^{-1} \mathbf{q}_0 \right] \right\} \\
&= \frac{(2\pi i)^{N/2}\sqrt{\det\left(\mathsf{D} - i\mathsf{B}\right)}}{\sqrt{\det \mathsf{B}}} \exp\left\{ \left[ -\frac{i}{2}\mathbf{q}^\intercal \mathsf{B}^{-1} + \frac{i}{2}\mathbf{Q}^\intercal \left(\mathsf{D} - i\mathsf{B}\right)\mathsf{B}^{-1} - \frac{1}{2}\mathbf{q}_0^\intercal \right] \left[ \left(\mathsf{D} - i\mathsf{B}\right)^{-\intercal} \mathbf{q} - \mathbf{Q} - i\mathsf{B}\left(\mathsf{D} - i\mathsf{B}\right)^{-1} \mathbf{q}_0 \right] \right\} \\
&= \frac{(2\pi i)^{N/2}\sqrt{\det\left(\mathsf{D} - i\mathsf{B}\right)}}{\sqrt{\det \mathsf{B}}} \exp\left[ -\frac{i}{2}\mathbf{q}^\intercal \mathsf{B}^{-1}\left(\mathsf{D} - i\mathsf{B}\right)^{-\intercal}\mathbf{q} - \frac{i}{2}\mathbf{Q}^\intercal \left(\mathsf{D}\mathsf{B}^{-1} - i\,\mathsf{I}_N\right)\mathbf{Q} + \frac{i}{2}\mathbf{q}_0^\intercal \mathsf{B}\left(\mathsf{D} - i\mathsf{B}\right)^{-1}\mathbf{q}_0 \right. \\
&\qquad\qquad \left. + i\mathbf{q}^\intercal \mathsf{B}^{-1}\mathbf{Q} - \mathbf{q}^\intercal \left(\mathsf{D} - i\mathsf{B}\right)^{-1}\mathbf{q}_0 + \mathbf{q}_0^\intercal \mathbf{Q} \right] , \qquad \text{(S22)}
\end{aligned}$$

where we have used Eq. (S11). Performing the integration over $\mathbf{q}_0$ then yields

$$\begin{aligned}
\psi(\mathbf{q}) &= \frac{\sigma \exp\left[ -\frac{1}{2}\mathbf{q}^\intercal \left(\mathsf{D} - i\mathsf{B}\right)^{-1}\left(\mathsf{A} + i\mathsf{C} + i\mathsf{B}^{-\intercal}\right)\mathbf{q}\right]}{(-2\pi i)^{N/2}\pi^{N/2}\sqrt{\det \mathsf{B}}} \\
&\quad \times \int \mathrm{d}\mathbf{Q}\,\mathrm{d}\mathbf{q}_0\,\Psi(\mathbf{Q}) \exp\left[ -\frac{i}{2}\mathbf{Q}^\intercal \left(\mathsf{D}\mathsf{B}^{-1} - 2i\,\mathsf{I}_N\right)\mathbf{Q} + i\mathbf{q}^\intercal \mathsf{B}^{-1}\mathbf{Q} - \mathbf{q}_0^\intercal \mathbf{q}_0 + 2\mathbf{q}_0^\intercal \mathbf{Q} \right] , \\
&= \frac{\sigma \exp\left[ -\frac{1}{2}\mathbf{q}^\intercal \left(\mathsf{D} - i\mathsf{B}\right)^{-1}\left(\mathsf{A} + i\mathsf{C} + i\mathsf{B}^{-\intercal}\right)\mathbf{q}\right]}{(-2\pi i)^{N/2}\sqrt{\det \mathsf{B}}} \int \mathrm{d}\mathbf{Q}\,\Psi(\mathbf{Q}) \exp\left[ -\frac{i}{2}\mathbf{Q}^\intercal \mathsf{D}\mathsf{B}^{-1}\mathbf{Q} + i\mathbf{q}^\intercal \mathsf{B}^{-1}\mathbf{Q} \right] . \qquad \text{(S23)}
\end{aligned}$$

Using Eqs. (A1a) and (A1c) of the main text, we can simplify

$$\mathsf{A} + i\mathsf{C} + i\mathsf{B}^{-\intercal} = \mathsf{A} + i(\mathsf{C}\mathsf{B}^\intercal + \mathsf{I}_N)\mathsf{B}^{-\intercal} = \mathsf{A} + i\mathsf{D}\mathsf{A}^\intercal\mathsf{B}^{-\intercal} = \mathsf{A} + i\mathsf{D}\mathsf{B}^{-1}\mathsf{A} = i(\mathsf{D} - i\mathsf{B})\mathsf{B}^{-1}\mathsf{A} , \qquad \text{(S24)}$$

thus obtaining the inverse MT.

### C. Saddlepoint calculation

There are two ways to calculate the saddlepoints of Eq. (S19). The first is to immediately compute the saddlepoints of Eq. (S19), while the second is to integrate over $\mathbf{q}_0$ first, then compute the saddlepoints of the resulting integral. Note that $\mathbf{p}_0$ cannot be integrated over without inverting $\mathsf{B}$.

#### 1. *Direct calculation of saddlepoints*

The (complex) phase of the integrand in Eq. (S19) is

$$i\Theta(\mathbf{Q}) - \frac{1}{2}\mathbf{Q}^\intercal\mathbf{Q} - \frac{i}{2}\boldsymbol{\zeta}^\intercal \mathsf{B}\left(\mathsf{D} - i\mathsf{B}\right)^{-1}\boldsymbol{\zeta} - \mathbf{q}_0^\intercal\mathbf{q}_0 + \mathbf{Q}^\intercal\boldsymbol{\zeta}^* + \mathbf{q}^\intercal\left(\mathsf{D} - i\mathsf{B}\right)^{-1}\boldsymbol{\zeta} . \qquad \text{(S25)}$$

This phase is a function of $\mathbf{Q}$, $\mathbf{p}_0$, and $\mathbf{q}_0$, so it is stationary when the derivatives of the phase with respect to all these variables are equal to zero simultaneously. Hence, we require $\mathbf{Q}$, $\mathbf{p}_0$, and $\mathbf{q}_0$ to simultaneously satisfy

$$i\left[\mathbf{P}(\mathbf{Q}) - \mathbf{p}_0\right] - \left(\mathbf{Q} - \mathbf{q}_0\right) = 0 , \qquad \text{(S26a)}$$

$$i\left(\mathsf{D} - i\mathsf{B}\right)^{-\intercal}\left[\mathbf{q} - \mathsf{D}^\intercal\mathbf{Q} + \mathsf{B}^\intercal\mathbf{p}_0 + i\mathsf{B}^\intercal\left(\mathbf{Q} - \mathbf{q}_0\right)\right] = 0 , \qquad \text{(S26b)}$$

$$\left(\mathsf{D} - i\mathsf{B}\right)^{-\intercal}\left[\mathbf{q} - \mathsf{D}^\intercal\mathbf{q}_0 + \mathsf{B}^\intercal\mathbf{p}_0 + \left(\mathsf{D} - i\mathsf{B}\right)^\intercal\left(\mathbf{Q} - \mathbf{q}_0\right)\right] = 0 . \qquad \text{(S26c)}$$

Let us restrict $\mathbf{P}(\mathbf{Q})$, $\mathbf{Q}$, $\mathbf{p}_0$, and $\mathbf{q}_0$ to all be purely real. Then, the first equation is solved by $\mathbf{q}_0 = \mathbf{Q}$, $\mathbf{p}_0 = \mathbf{P}(\mathbf{Q})$. Since $\mathsf{D} - i\mathsf{B}$ is invertible, the other two equations both reduce to

$$\mathbf{q} = \mathsf{D}^\intercal\mathbf{Q} - \mathsf{B}^\intercal\mathbf{P}(\mathbf{Q}) . \qquad \text{(S27)}$$

When $\mathbf{q} = \mathbf{q}(\mathbf{t})$, then this equation can be satisfied at $\mathbf{Q} = \mathbf{Q}(\mathbf{t})$ by definition of the rotated rays [Eqs. (24) from the main text][2]. Hence, the phase is stationary where

$$\mathbf{Q} = \mathbf{Q}(\mathbf{t}) \, , \quad \mathbf{q}_0 = \mathbf{Q}(\mathbf{t}) \, , \quad \mathbf{p}_0 = \mathbf{P}(\mathbf{t}) \, . \tag{S28}$$

Let us make the variable substitutions

$$\boldsymbol{\epsilon} \doteq \mathbf{Q} - \mathbf{Q}(\mathbf{t}) \, , \quad \boldsymbol{\xi} \doteq \boldsymbol{\zeta} - \boldsymbol{\zeta}(\mathbf{t}) \, , \quad \boldsymbol{\zeta}(\mathbf{t}) \doteq \mathbf{Q}(\mathbf{t}) + i\mathbf{P}(\mathbf{t}) \, , \tag{S29}$$

so $\boldsymbol{\xi}_r \doteq \mathrm{Re}(\boldsymbol{\xi})$ and $\boldsymbol{\xi}_i \doteq \mathrm{Im}(\boldsymbol{\xi})$ are given by

$$\boldsymbol{\xi}_r = \mathbf{q}_0 - \mathbf{Q}(\mathbf{t}) \, , \quad \boldsymbol{\xi}_i = \mathbf{p}_0 - \mathbf{P}(\mathbf{t}) \, . \tag{S30}$$

Then, since

$$\Psi(\mathbf{Q}) = \Psi\left[\boldsymbol{\epsilon} + \mathbf{Q}(\mathbf{t})\right] \, , \tag{S31a}$$

$$-\frac{1}{2}\mathbf{Q}^\intercal\mathbf{Q} = -\frac{1}{2}\boldsymbol{\epsilon}^\intercal\boldsymbol{\epsilon} - \boldsymbol{\epsilon}^\intercal\mathbf{Q}(\mathbf{t}) - \frac{1}{2}\mathbf{Q}^\intercal(\mathbf{t})\mathbf{Q}(\mathbf{t}) \, , \tag{S31b}$$

$$-\frac{i}{2}\boldsymbol{\zeta}^\intercal\mathsf{B}\left(\mathsf{D} - i\mathsf{B}\right)^{-1}\boldsymbol{\zeta} = -\frac{i}{2}\boldsymbol{\xi}^\intercal\mathsf{B}\left(\mathsf{D} - i\mathsf{B}\right)^{-1}\boldsymbol{\xi} - i\boldsymbol{\xi}^\intercal\mathsf{B}\left(\mathsf{D} - i\mathsf{B}\right)^{-1}\boldsymbol{\zeta}(\mathbf{t}) - \frac{i}{2}\boldsymbol{\zeta}^\intercal(\mathbf{t})\mathsf{B}\left(\mathsf{D} - i\mathsf{B}\right)^{-1}\boldsymbol{\zeta}(\mathbf{t}) \, , \tag{S31c}$$

$$-\mathbf{q}_0^\intercal\mathbf{q}_0 = -\boldsymbol{\xi}_r^\intercal\boldsymbol{\xi}_r - 2\boldsymbol{\xi}_r^\intercal\mathbf{Q}(\mathbf{t}) - \mathbf{Q}^\intercal(\mathbf{t})\mathbf{Q}(\mathbf{t}) \, , \tag{S31d}$$

$$+\mathbf{Q}^\intercal\boldsymbol{\zeta}^* = +\boldsymbol{\epsilon}^\intercal\boldsymbol{\xi}^* + \boldsymbol{\epsilon}^\intercal\boldsymbol{\zeta}^*(\mathbf{t}) + \mathbf{Q}^\intercal(\mathbf{t})\boldsymbol{\xi}^* + \mathbf{Q}^\intercal(\mathbf{t})\boldsymbol{\zeta}^*(\mathbf{t}) \, , \tag{S31e}$$

$$+\mathbf{q}^\intercal\left(\mathsf{D} - i\mathsf{B}\right)^{-1}\boldsymbol{\zeta} = +\mathbf{q}^\intercal\left(\mathsf{D} - i\mathsf{B}\right)^{-1}\boldsymbol{\xi} + \mathbf{q}^\intercal\left(\mathsf{D} - i\mathsf{B}\right)^{-1}\boldsymbol{\zeta}(\mathbf{t}) \, , \tag{S31f}$$

we obtain

$$\begin{aligned}
\psi(\mathbf{q}) = &\frac{\sigma \exp\left[-\frac{1}{2}\mathbf{q}^\intercal\left(\mathsf{D} - i\mathsf{B}\right)^{-1}\left(\mathsf{A} + i\mathsf{C}\right)\mathbf{q} - \frac{3}{2}\mathbf{Q}^\intercal(\mathbf{t})\mathbf{Q}(\mathbf{t}) - \frac{i}{2}\boldsymbol{\zeta}^\intercal(\mathbf{t})\mathsf{B}\left(\mathsf{D} - i\mathsf{B}\right)^{-1}\boldsymbol{\zeta}(\mathbf{t}) + \mathbf{Q}^\intercal(\mathbf{t})\boldsymbol{\zeta}^*(\mathbf{t}) + \mathbf{q}^\intercal\left(\mathsf{D} - i\mathsf{B}\right)^{-1}\boldsymbol{\zeta}(\mathbf{t})\right]}{(2\pi)^N\pi^{N/2}\sqrt{\det(\mathsf{D} - i\mathsf{B})}} \\
&\times \int \mathrm{d}\boldsymbol{\epsilon}\,\mathrm{d}\boldsymbol{\xi}_r\,\mathrm{d}\boldsymbol{\xi}_i\,\Psi[\boldsymbol{\epsilon} + \mathbf{Q}(\mathbf{t})]\exp\left\{-\frac{1}{2}\boldsymbol{\epsilon}^\intercal\boldsymbol{\epsilon} + \boldsymbol{\epsilon}^\intercal\left[\boldsymbol{\xi}^* + \boldsymbol{\zeta}^*(\mathbf{t}) - \mathbf{Q}(\mathbf{t})\right] - \boldsymbol{\xi}_r^\intercal\boldsymbol{\xi}_r - 2\boldsymbol{\xi}_r^\intercal\mathbf{Q}(\mathbf{t}) + \mathbf{Q}^\intercal(\mathbf{t})\boldsymbol{\xi}^* \right. \\
&\left. \qquad - \frac{i}{2}\boldsymbol{\xi}^\intercal\mathsf{B}\left(\mathsf{D} - i\mathsf{B}\right)^{-1}\boldsymbol{\xi} + \boldsymbol{\xi}^\intercal\left(\mathsf{D} - i\mathsf{B}\right)^{-\intercal}\left[\mathbf{q} - i\mathsf{B}^\intercal\boldsymbol{\zeta}(\mathbf{t})\right]\right\} \, ,
\end{aligned} \tag{S32}$$

where the saddlepoint is now located at $\boldsymbol{\epsilon} = \boldsymbol{\xi} = 0$.

### *2. Integration, then calculation of saddlepoints*

Let us perform the integration over $\mathbf{q}_0$. This involves inverting $2\mathsf{D} - i\mathsf{B}$, and one can show that $\det(2\mathsf{D} - i\mathsf{B}) \neq 0$ by the same proof as presented in Ref. [2, p. 2956]. We then compute

$$\begin{aligned}
&\int \mathrm{d}\mathbf{q}_0 \, \exp\left\{-\frac{1}{2}\mathbf{q}_0^\intercal\left(2\mathsf{D} - i\mathsf{B}\right)\left(\mathsf{D} - i\mathsf{B}\right)^{-1}\mathbf{q}_0 + \mathbf{q}_0^\intercal\left[\left(\mathsf{D} - i\mathsf{B}\right)^{-\intercal}\mathbf{q} + \mathbf{Q} + \mathsf{B}\left(\mathsf{D} - i\mathsf{B}\right)^{-1}\mathbf{p}_0\right]\right\} \\
&= \frac{(2\pi)^{N/2}\sqrt{\det(\mathsf{D} - i\mathsf{B})}}{\sqrt{\det(2\mathsf{D} - i\mathsf{B})}} \, \exp\left\{\frac{1}{2}\left[\mathbf{q}^\intercal\left(2\mathsf{D} - i\mathsf{B}\right)^{-1} + \mathbf{Q}^\intercal\left(\mathsf{D} - i\mathsf{B}\right)\left(2\mathsf{D} - i\mathsf{B}\right)^{-1} + \mathbf{p}_0^\intercal\mathsf{B}\left(2\mathsf{D} - i\mathsf{B}\right)^{-1}\right]^\intercal \right. \\
&\qquad \left. \times \left[\left(\mathsf{D} - i\mathsf{B}\right)^{-\intercal}\mathbf{q} + \mathbf{Q} + \mathsf{B}\left(\mathsf{D} - i\mathsf{B}\right)^{-1}\mathbf{p}_0\right]\right\} \\
&= \frac{(2\pi)^{N/2}\sqrt{\det(\mathsf{D} - i\mathsf{B})}}{\sqrt{\det(2\mathsf{D} - i\mathsf{B})}} \, \exp\left\{\frac{1}{2}\mathbf{q}^\intercal\left(2\mathsf{D} - i\mathsf{B}\right)^{-1}\left(\mathsf{D} - i\mathsf{B}\right)^{-\intercal}\mathbf{q} + \frac{1}{2}\mathbf{Q}^\intercal\left(\mathsf{D} - i\mathsf{B}\right)\left(2\mathsf{D} - i\mathsf{B}\right)^{-1}\mathbf{Q} + \mathbf{q}^\intercal\left(2\mathsf{D} - i\mathsf{B}\right)^{-1}\mathbf{Q} \right. \\
&\qquad \left. + \frac{1}{2}\mathbf{p}_0^\intercal\mathsf{B}\left(2\mathsf{D} - i\mathsf{B}\right)^{-1}\left(\mathsf{D} - i\mathsf{B}\right)^{-\intercal}\mathsf{B}^\intercal\mathbf{p}_0 + \mathbf{p}_0^\intercal\mathsf{B}\left(2\mathsf{D} - i\mathsf{B}\right)^{-1}\left[\left(\mathsf{D} - i\mathsf{B}\right)^{-\intercal}\mathbf{q} + \mathbf{Q}\right]\right\} \, .
\end{aligned} \tag{S33}$$

[2] However, note that additional roots are possible depending on the details of $\mathsf{S}$ and $\mathbf{P}(\mathbf{Q})$.

Hence,

$$\psi(\mathbf{q}) = \frac{\sigma \exp\left[-\frac{1}{2}\mathbf{q}^\intercal \left(2\mathsf{D} - i\mathsf{B}\right)^{-1}\left(\mathsf{A} + 2i\mathsf{C}\right)\mathbf{q}\right]}{(\sqrt{2}\,\pi)^N\sqrt{\det(2\mathsf{D} - i\mathsf{B})}} \times \int \mathrm{d}\mathbf{Q}\,\mathrm{d}\mathbf{p}_0\,\Psi(\mathbf{Q})\exp\left[-\frac{1}{2}\boldsymbol{\xi}^\intercal\mathsf{D}\left(2\mathsf{D} - i\mathsf{B}\right)^{-1}\boldsymbol{\xi} + \mathbf{q}^\intercal\left(2\mathsf{D} - i\mathsf{B}\right)^{-1}\boldsymbol{\xi} - \mathbf{p}_0^\intercal\mathbf{p}_0\right], \tag{S34}$$

where we have defined the complex vector $\boldsymbol{\xi} \doteq \mathbf{Q} + 2i\mathbf{p}_0$. The (complex) phase of the integrand of Eq. (S34) is

$$i\Theta(\mathbf{Q}) - \frac{1}{2}\mathbf{Q}^\intercal\mathsf{D}\left(2\mathsf{D} - i\mathsf{B}\right)^{-1}\mathbf{Q} + \mathbf{q}^\intercal\left(2\mathsf{D} - i\mathsf{B}\right)^{-1}\mathbf{Q} + i\mathbf{p}_0^\intercal\mathsf{B}\left(2\mathsf{D} - i\mathsf{B}\right)^{-1}\mathbf{p}_0 + 2i\mathbf{p}_0^\intercal\left(2\mathsf{D} - i\mathsf{B}\right)^{-\intercal}\left(\mathbf{q} - \mathsf{D}^\intercal\mathbf{Q}\right). \tag{S35}$$

Since the phase is a function of $\mathbf{Q}$ and $\mathbf{p}_0$, it is stationary when the derivatives of the phase with respect to both these variables vanish simultaneously. Hence, we require $\mathbf{Q}$ and $\mathbf{p}_0$ to simultaneously satisfy

$$\left(2\mathsf{D} - i\mathsf{B}\right)^{-\intercal}\left\{2i\mathsf{D}^\intercal\left[\mathbf{P}(\mathbf{Q}) - \mathbf{p}_0\right] + \mathbf{q} - \mathsf{D}^\intercal\mathbf{Q} + \mathsf{B}^\intercal\mathbf{P}(\mathbf{Q})\right\} = 0\,, \tag{S36a}$$

$$2i\left(2\mathsf{D} - i\mathsf{B}\right)^{-\intercal}\left(\mathbf{q} - \mathsf{D}^\intercal\mathbf{Q} + \mathsf{B}^\intercal\mathbf{p}_0\right) = 0\,. \tag{S36b}$$

By the same logic as with Eqs. (S26), we obtain as a simultaneous solution

$$\mathbf{Q} = \mathbf{Q}(\mathbf{t})\,, \quad \mathbf{p}_0 = \mathbf{P}(\mathbf{t})\,. \tag{S37}$$

Let us define

$$\boldsymbol{\xi}(\mathbf{t}) \doteq \mathbf{Q}(\mathbf{t}) + 2i\mathbf{P}(\mathbf{t})\,, \quad \boldsymbol{\epsilon} \doteq \boldsymbol{\xi} - \boldsymbol{\xi}(\mathbf{t})\,, \tag{S38}$$

so that $\boldsymbol{\epsilon}_r \doteq \mathrm{Re}(\boldsymbol{\epsilon})$ and $\boldsymbol{\epsilon}_i \doteq \mathrm{Im}(\boldsymbol{\epsilon})$ are given by

$$\boldsymbol{\epsilon}_r = \mathbf{Q} - \mathbf{Q}(\mathbf{t})\,, \quad \boldsymbol{\epsilon}_i = 2\mathbf{p}_0 - 2\mathbf{P}(\mathbf{t})\,. \tag{S39}$$

Consequently,

$$\mathrm{d}\mathbf{Q} = \mathrm{d}\boldsymbol{\epsilon}_r\,, \quad \mathrm{d}\mathbf{p}_0 = 2^{-N}\mathrm{d}\boldsymbol{\epsilon}_i\,. \tag{S40}$$

Then, since

$$-\frac{1}{2}\boldsymbol{\xi}^\intercal\mathsf{D}\left(2\mathsf{D} - i\mathsf{B}\right)^{-1}\boldsymbol{\xi} = -\frac{1}{2}\boldsymbol{\epsilon}^\intercal\mathsf{D}\left(2\mathsf{D} - i\mathsf{B}\right)^{-1}\boldsymbol{\epsilon} - \boldsymbol{\epsilon}^\intercal\mathsf{D}\left(2\mathsf{D} - i\mathsf{B}\right)^{-1}\boldsymbol{\xi}(\mathbf{t}) - \frac{1}{2}\boldsymbol{\xi}^\intercal(\mathbf{t})\mathsf{D}\left(2\mathsf{D} - i\mathsf{B}\right)^{-1}\boldsymbol{\xi}(\mathbf{t})\,, \tag{S41a}$$

$$+\mathbf{q}^\intercal\left(2\mathsf{D} - i\mathsf{B}\right)^{-1}\boldsymbol{\xi} = +\mathbf{q}^\intercal\left(2\mathsf{D} - i\mathsf{B}\right)^{-1}\boldsymbol{\epsilon} + \mathbf{q}^\intercal\left(2\mathsf{D} - i\mathsf{B}\right)^{-1}\boldsymbol{\xi}(\mathbf{t})\,, \tag{S41b}$$

$$-\mathbf{p}_0^\intercal\mathbf{p}_0 = -\frac{1}{4}\boldsymbol{\epsilon}_i^\intercal\boldsymbol{\epsilon}_i - \boldsymbol{\epsilon}_i^\intercal\mathbf{P}(\mathbf{t}) - \mathbf{P}^\intercal(\mathbf{t})\mathbf{P}(\mathbf{t})\,, \tag{S41c}$$

we obtain

$$\psi(\mathbf{q}) = \frac{\sigma\exp\left[-\frac{1}{2}\mathbf{q}^\intercal\left(2\mathsf{D} - i\mathsf{B}\right)^{-1}\left(\mathsf{A} + 2i\mathsf{C}\right)\mathbf{q} - \frac{1}{2}\boldsymbol{\xi}^\intercal(\mathbf{t})\mathsf{D}\left(2\mathsf{D} - i\mathsf{B}\right)^{-1}\boldsymbol{\xi}(\mathbf{t}) + \mathbf{q}^\intercal\left(2\mathsf{D} - i\mathsf{B}\right)^{-1}\boldsymbol{\xi}(\mathbf{t}) - \mathbf{P}^\intercal(\mathbf{t})\mathbf{P}(\mathbf{t})\right]}{(2\sqrt{2}\,\pi)^N\sqrt{\det(2\mathsf{D} - i\mathsf{B})}} \times \int \mathrm{d}\boldsymbol{\epsilon}_r\,\mathrm{d}\boldsymbol{\epsilon}_i\,\Psi[\boldsymbol{\epsilon}_r + \mathbf{Q}(\mathbf{t})]\exp\left\{-\frac{1}{2}\boldsymbol{\epsilon}^\intercal\mathsf{D}\left(2\mathsf{D} - i\mathsf{B}\right)^{-1}\boldsymbol{\epsilon} + \boldsymbol{\epsilon}^\intercal\left(2\mathsf{D} - i\mathsf{B}\right)^{-\intercal}\left[\mathbf{q} - \mathsf{D}^\intercal\boldsymbol{\xi}(\mathbf{t})\right] - \frac{1}{4}\boldsymbol{\epsilon}_i^\intercal\boldsymbol{\epsilon}_i - \boldsymbol{\epsilon}_i^\intercal\mathbf{P}(\mathbf{t})\right\}, \tag{S42}$$

where the saddlepoint is now located at $\boldsymbol{\epsilon} = \mathbf{0}$.

## Appendix: Derivation of some basic properties of coherent states

Coherent states $|\mathbf{z}_0\rangle$ are normalized to unity:

$$\begin{aligned}\langle\mathbf{z}_0|\mathbf{z}_0\rangle &= \int \mathrm{d}\mathbf{q}\,\langle\mathbf{z}_0|\mathbf{q}\rangle\langle\mathbf{q}|\mathbf{z}_0\rangle = \int \mathrm{d}\mathbf{q}\,\langle\mathbf{z}_0|\mathbf{q}\rangle(\langle\mathbf{z}_0|\mathbf{q}\rangle)^* \\ &= \int \mathrm{d}\mathbf{q}\,\pi^{-N/4}\exp\left[-\frac{1}{2}(\mathbf{q}')^\intercal\mathbf{q}' + (\mathbf{q}')^\intercal\boldsymbol{\zeta}^* - \frac{1}{4}(\boldsymbol{\zeta} + \boldsymbol{\zeta}^*)^\intercal\boldsymbol{\zeta}^*\right]\pi^{-N/4}\exp\left[-\frac{1}{2}(\mathbf{q}')^\intercal\mathbf{q}' + (\mathbf{q}')^\intercal\boldsymbol{\zeta} - \frac{1}{4}(\boldsymbol{\zeta} + \boldsymbol{\zeta}^*)^\intercal\boldsymbol{\zeta}\right] \\ &= \frac{1}{\pi^{N/2}}\int \mathrm{d}\mathbf{q}\,\exp\left[-(\mathbf{q} - \mathbf{q}_0)^\intercal(\mathbf{q} - \mathbf{q}_0)\right] = 1\,.\end{aligned} \tag{S43}$$

Also, the expectation value of $\hat{\mathbf{z}} \doteq (\hat{\mathbf{q}}, \hat{\mathbf{p}})^\intercal$ is $\mathbf{z}_0 \doteq (\mathbf{q}_0, \mathbf{p}_0)^\intercal$, which is seen as follows:

$$\begin{aligned}\langle \mathbf{z}_0 | \hat{\mathbf{q}} | \mathbf{z}_0 \rangle &= \int \mathrm{d}\mathbf{q} \, \langle \mathbf{z}_0 | \mathbf{q} \rangle \, \langle \mathbf{q} | \hat{\mathbf{q}} | \mathbf{z}_0 \rangle = \int \mathrm{d}\mathbf{q} \, \langle \mathbf{z}_0 | \mathbf{q} \rangle \, \mathbf{q} \langle \mathbf{q} | \mathbf{z}_0 \rangle = \frac{1}{\pi^{N/2}} \int \mathrm{d}\mathbf{q} \, \mathbf{q} \exp\left[ -(\mathbf{q} - \mathbf{q}_0)^\intercal (\mathbf{q} - \mathbf{q}_0) \right] \\ &= \frac{\pi^{N/2} \, \mathbf{q}_0}{\pi^{N/2}} = \mathbf{q}_0 \, , \end{aligned} \tag{S44}$$

$$\begin{aligned}\langle \mathbf{z}_0 | \hat{\mathbf{p}} | \mathbf{z}_0 \rangle &= \int \mathrm{d}\mathbf{q} \, \langle \mathbf{z}_0 | \mathbf{q} \rangle \, \langle \mathbf{q} | \hat{\mathbf{p}} | \mathbf{z}_0 \rangle = \int \mathrm{d}\mathbf{q} \, \langle \mathbf{z}_0 | \mathbf{q} \rangle \left( -i \partial_{\mathbf{q}} \langle \mathbf{q} | \mathbf{z}_0 \rangle \right) \\ &= \frac{-i}{\pi^{N/2}} \int \mathrm{d}\mathbf{q} \, (\mathbf{q}_0 + i\mathbf{p}_0 - \mathbf{q}) \exp\left[ -(\mathbf{q} - \mathbf{q}_0)^\intercal (\mathbf{q} - \mathbf{q}_0) \right] = \frac{-i}{\pi^{N/2}} \, i \pi^{N/2} \mathbf{p}_0 = \mathbf{p}_0 \, . \end{aligned} \tag{S45}$$

Finally, for any $|\psi\rangle$, one has

$$\begin{aligned} &\int \frac{\mathrm{d}\mathbf{q}_0 \, \mathrm{d}\mathbf{p}_0}{(2\pi)^N} \, \langle \psi | \mathbf{z}_0 \rangle \, \langle \mathbf{z}_0 | \psi \rangle = \int \frac{\mathrm{d}\mathbf{q}_0 \, \mathrm{d}\mathbf{p}_0 \, \mathrm{d}\mathbf{q}}{(2\pi)^N} \, \langle \psi | \mathbf{q} \rangle \, \langle \mathbf{q} | \mathbf{z}_0 \rangle \, \langle \mathbf{z}_0 | \psi \rangle \\ &= \int \frac{\mathrm{d}\mathbf{q}_0 \, \mathrm{d}\mathbf{p}_0 \, \mathrm{d}\mathbf{q}}{(2\pi)^N \pi^{N/4}} \, \langle \psi | \mathbf{q} \rangle \, \langle \mathbf{z}_0 | \psi \rangle \, \exp\left[ -\frac{1}{2} (\mathbf{q} - \mathbf{q}_0)^\intercal (\mathbf{q} - \mathbf{q}_0) + i \mathbf{p}_0^\intercal \mathbf{q} - \frac{i}{2} \mathbf{p}_0^\intercal \mathbf{q}_0 \right] \\ &= \int \frac{\mathrm{d}\mathbf{q}_0 \, \mathrm{d}\mathbf{p}_0 \, \mathrm{d}\mathbf{q} \, \mathrm{d}\mathbf{q}'}{(2\pi)^N \pi^{N/4}} \, \langle \psi | \mathbf{q} \rangle \, \langle \mathbf{z}_0 | \mathbf{q}' \rangle \langle \mathbf{q}' | \psi \rangle \, \exp\left[ -\frac{1}{2} (\mathbf{q} - \mathbf{q}_0)^\intercal (\mathbf{q} - \mathbf{q}_0) + i \mathbf{p}_0^\intercal \mathbf{q} - \frac{i}{2} \mathbf{p}_0^\intercal \mathbf{q}_0 \right] \\ &= \int \frac{\mathrm{d}\mathbf{q}_0 \, \mathrm{d}\mathbf{p}_0 \, \mathrm{d}\mathbf{q} \, \mathrm{d}\mathbf{q}'}{(2\pi)^N \pi^{N/2}} \, \langle \psi | \mathbf{q} \rangle \, \langle \mathbf{q}' | \psi \rangle \, \exp\left[ -\frac{1}{2} (\mathbf{q} - \mathbf{q}_0)^\intercal (\mathbf{q} - \mathbf{q}_0) - \frac{1}{2} (\mathbf{q}' - \mathbf{q}_0)^\intercal (\mathbf{q}' - \mathbf{q}_0) + i \mathbf{p}_0^\intercal (\mathbf{q} - \mathbf{q}') \right] \\ &= \int \frac{\mathrm{d}\mathbf{q}_0 \, \mathrm{d}\mathbf{q} \, \mathrm{d}\mathbf{q}'}{(2\pi)^N \pi^{N/2}} \, \langle \psi | \mathbf{q} \rangle \, \langle \mathbf{q}' | \psi \rangle \, \exp\left[ -\frac{1}{2} (\mathbf{q} - \mathbf{q}_0)^\intercal (\mathbf{q} - \mathbf{q}_0) - \frac{1}{2} (\mathbf{q}' - \mathbf{q}_0)^\intercal (\mathbf{q}' - \mathbf{q}_0) \right] \int \mathrm{d}\mathbf{p}_0 \, \exp\left[ i \mathbf{p}_0^\intercal (\mathbf{q} - \mathbf{q}') \right] \\ &= \int \frac{\mathrm{d}\mathbf{q}_0 \, \mathrm{d}\mathbf{q} \, \mathrm{d}\mathbf{q}'}{(2\pi)^N \pi^{N/2}} \, \langle \psi | \mathbf{q} \rangle \, \langle \mathbf{q}' | \psi \rangle \, \exp\left[ -\frac{1}{2} (\mathbf{q} - \mathbf{q}_0)^\intercal (\mathbf{q} - \mathbf{q}_0) - \frac{1}{2} (\mathbf{q}' - \mathbf{q}_0)^\intercal (\mathbf{q}' - \mathbf{q}_0) \right] (2\pi)^N \delta(\mathbf{q} - \mathbf{q}') \\ &= \int \frac{\mathrm{d}\mathbf{q}}{\pi^{N/2}} \, \langle \psi | \mathbf{q} \rangle \, \langle \mathbf{q} | \psi \rangle \int \mathrm{d}\mathbf{q}_0 \, \exp\left[ -(\mathbf{q} - \mathbf{q}_0)^\intercal (\mathbf{q} - \mathbf{q}_0) \right] \\ &= \int \mathrm{d}\mathbf{q} \, \langle \psi | \mathbf{q} \rangle \, \langle \mathbf{q} | \psi \rangle = \langle \psi | \psi \rangle \, , \end{aligned} \tag{S46}$$

which proves the completeness relation (S4).

## II. METAPLECTIC GEOMETRICAL OPTICS EXAMPLES

### A. Plane wave in free space

Consider a plane wave propagating along $+q$ direction in a homogeneous medium, which we take to be one-dimensional without loss of generality. The corresponding governing equation is

$$i\partial_q \psi(q) + \psi(q) = 0 \, . \tag{S47}$$

This equation has the exact solution

$$\psi(q) = c e^{iq} \, , \tag{S48}$$

where $c$ is an arbitrary constant.

#### 1. *Weyl symbol*

We can equivalently write the wave equation as follows:

$$-\left( i\partial_q + 1 \right) \int \mathrm{d}q' \, \delta(q - q') \psi(q') = \int \mathrm{d}q' \, \left[ -i\partial_q \delta(q - q') - \delta(q - q') \right] \psi(q') = 0 \, , \tag{S49}$$

so the integration kernel is

$$D(q,q') = -i\delta'(q-q') - \delta(q-q') \,. \tag{S50}$$

Thus, we compute the dispersion symbol as

$$\begin{aligned}\mathcal{D}(q,k) = \int \mathrm{d}s\, e^{iks}\, D(q-s/2, q+s/2) &= \int \mathrm{d}s\, e^{iks}\, [-i\delta'(-s) - \delta(-s)] \\ &= \int \mathrm{d}s\, e^{-iks}\, [-i\delta'(s) - \delta(s)] \\ &= k - 1 \,. \end{aligned} \tag{S51}$$

## 2. Ray tracing

The ray equations for this system are

$$\partial_\tau k(\tau) = -\partial_q \mathcal{D}[q(\tau), k(\tau)] = 0 \,, \quad \partial_\tau q(\tau) = \partial_k \mathcal{D}[q(\tau), k(\tau)] = 1 \,. \tag{S52}$$

Hence, the solutions are

$$k(\tau) = k_0 \,, \quad q(\tau) = q_0 + \tau \,, \tag{S53}$$

where $k_0$ and $q_0$ are constants determined by initial conditions. We can take $q_0 = 0$ without loss of generality. Also, $\mathcal{D}(q_0, k_0) = 0$ requires $k_0 = 1$. Then, Eqs. (S52) lead to

$$k(\tau) = 1 \,, \quad q(\tau) = \tau \,, \tag{S54}$$

or in a vector form,

$$\mathbf{z}(\tau) = \begin{pmatrix} \tau \\ 1 \end{pmatrix} \,. \tag{S55}$$

By inverting Eqs. (S53), we also obtain $\tau$ and $k$ as functions of $q$:

$$\tau(q) = q \,, \quad k(q) = k[\tau(q)] = 1 \,. \tag{S56}$$

## 3. Tangent-space transformation matrix

We perform the symplectic Gram–Schmidt algorithm to compute $\mathsf{S}_t$ [3]. We calculate

$$\check{\mathbf{T}}_1(t) \doteq \frac{\partial_\tau \mathbf{z}(t)}{\|\partial_\tau \mathbf{z}(t)\|} = \begin{pmatrix} 1 \\ 0 \end{pmatrix} \,, \tag{S57}$$

which implies that

$$\check{\mathbf{N}}_1(t) \doteq -\mathsf{J}\, \check{\mathbf{T}}_1(t) = \begin{pmatrix} 0 & -1 \\ 1 & 0 \end{pmatrix} \begin{pmatrix} 1 \\ 0 \end{pmatrix} = \begin{pmatrix} 0 \\ 1 \end{pmatrix} \,. \tag{S58}$$

Hence, we obtain

$$\mathsf{S}_t = \begin{pmatrix} \check{\mathbf{T}}_1^\intercal(t) \\ \check{\mathbf{N}}_1^\intercal(t) \end{pmatrix} = \mathsf{I}_2 \,, \tag{S59}$$

and correspondingly,

$$\mathsf{A}_t = 1 \,, \quad \mathsf{B}_t = 0 \,, \quad \mathsf{C}_t = 0 \,, \quad \mathsf{D}_t = 1 \,. \tag{S60}$$

### *4. Tangent-space rays*

The tangent-space rays are obtained as

$$Q_t(\tau) = \mathsf{A}_t\, q(\tau) + \mathsf{B}_t\, k(\tau) = \tau\,, \quad K_t(\tau) = \mathsf{C}_t\, q(\tau) + \mathsf{D}_t\, k(\tau) = 1\,. \tag{S61}$$

Hence,

$$\tau_t(Q) = Q\,, \quad K_t(Q) = K_t[\tau_t(Q)] = 1\,. \tag{S62}$$

### *5. Tangent-space phase*

The wave phase on the tangent space is

$$\Theta_t(Q) = \int_{Q_t(t)}^{Q} \mathrm{d}Q\, K_t(Q) = Q - Q_t(t) = Q - t\,, \tag{S63}$$

where we have used $Q_t(t) = t$. In terms of $\epsilon \doteq Q - Q_t(t)$, we obtain

$$\Theta_t[\epsilon + Q_t(t)] = \epsilon\,. \tag{S64}$$

### *6. Tangent-space envelope*

The group velocity on the tangent space is

$$V_t(Q) = \partial_K \mathcal{D}(\mathsf{S}_t^{-1} \boldsymbol{\mathsf{Z}}_t) = 1\,. \tag{S65}$$

Hence, $\partial_Q V_t(Q) = 0$ and the envelope equation is

$$\partial_Q \Phi_t(Q) = 0\,. \tag{S66}$$

The solution that satisfies $\Phi_t[Q_t(t)] = 1$ is thus

$$\Phi_t[\epsilon + Q_t(t)] = 1\,. \tag{S67}$$

### *7. Linking with NIMT*

To compute $\alpha_t$, we must first compute

$$\eta_t \doteq \Big[\partial_t Q_t(t) - \mathsf{V}_t Q_t(t)\Big] \Big\{\partial_Q \Phi_t\left[Q_t(t)\right] + i K_t(t)\Big\} - K_t(t) \mathsf{W}_t \left\{\partial_Q \Phi_t\left[Q_t(t)\right] + \frac{i}{2} K_t(t)\right\} - \frac{1}{2}\mathsf{V}_t - \frac{i}{2}\mathsf{U}_t Q_t^2(t)\,. \tag{S68}$$

Since $\mathsf{S}_t = \mathsf{I}_2$, one has $\partial_t \mathsf{S}_t = \mathsf{0}_2$, and consequently,

$$\begin{pmatrix} \mathsf{V}_t & \mathsf{W}_t \\ -\mathsf{U}_t & -\mathsf{V}_t \end{pmatrix} \doteq (\partial_t \mathsf{S}_t)\, \mathsf{S}_t^{-1} = \mathsf{0}_2\,. \tag{S69}$$

Hence, we obtain the simplification

$$\eta_t = \partial_t Q_t(t) \Big\{\partial_Q \Phi_t\left[Q_t(t)\right] + i K_t(t)\Big\}\,. \tag{S70}$$

Next, since $\Phi_t(Q) = 1$, one has $\partial_Q \Phi_t\left[Q_t(t)\right] = 0$, and we obtain

$$\eta_t = i \partial_t Q_t(t) K_t(t)\,. \tag{S71}$$

Lastly, since $K_t(t) = 1$ and $Q_t(t) = t$, we obtain

$$\eta_t = i\,. \tag{S72}$$

Therefore, we also obtain

$$\alpha_t = \alpha_0 \exp\left(\int_0^t \mathrm{d}\tau\, \eta_\tau\right) = \alpha_0 \exp(it)\,, \tag{S73}$$

where $\alpha_0$ is a constant.

*8. Inverse MT*

Since $B_t = 0$, we have $\rho = 0$. Thus,

$$\mathsf{a}_{\rho\rho} = \mathsf{a}_{\rho\varsigma} = (\cdot)\,, \quad \mathsf{a}_{\varsigma\varsigma} = 1\,, \tag{S74a}$$

$$\Lambda_{\rho\rho} = (\cdot)\,, \tag{S74b}$$

$$\mathsf{c}_{\rho\rho} = \mathsf{c}_{\rho\varsigma} = \mathsf{c}_{\varsigma\rho} = (\cdot)\,, \quad \mathsf{c}_{\varsigma\varsigma} = 0\,, \tag{S74c}$$

$$\mathsf{d}_{\rho\rho} = \mathsf{d}_{\varsigma\rho} = (\cdot)\,, \quad \mathsf{d}_{\varsigma\varsigma} = 1\,, \tag{S74d}$$

where $(\cdot)$ denotes an empty matrix. Note that $(\cdot) \neq 0_1$, because while $(\cdot)\mathsf{M} = (\cdot)$ for any $\mathsf{M}$, $\det(\cdot) = 1$ by our convention. We compute

$$\mathsf{M}_3 \doteq \begin{pmatrix} \Lambda_{\rho\rho}^{-1} & -\Lambda_{\rho\rho}^{-1}\mathsf{d}_{\varsigma\rho}^\intercal \mathsf{a}_{\varsigma\varsigma} \end{pmatrix} = (\cdot)\,, \tag{S75}$$

$$\mathsf{M}_4 \doteq \begin{pmatrix} \Lambda_{\rho\rho}^{-1}\mathsf{a}_{\rho\rho} & \Lambda_{\rho\rho}^{-1}\mathsf{a}_{\rho\varsigma} \\ \mathsf{a}_{\rho\varsigma}^\intercal \Lambda_{\rho\rho}^{-1} & \mathsf{a}_{\varsigma\varsigma}^\intercal \mathsf{c}_{\varsigma\varsigma} - \mathsf{a}_{\varsigma\varsigma}^\intercal \mathsf{d}_{\varsigma\rho}\Lambda_{\rho\rho}^{-1}\mathsf{a}_{\rho\varsigma} \end{pmatrix} = 0\,. \tag{S76}$$

Therefore,

$$\gamma_{\mathbf{t}}^{\rho}(\boldsymbol{\epsilon}_\rho, \mathbf{q}) \doteq \frac{1}{2}\boldsymbol{\epsilon}_\rho^\intercal \,\mathsf{d}_{\rho\rho}\Lambda_{\rho\rho}^{-1}\,\boldsymbol{\epsilon}_\rho + \boldsymbol{\epsilon}_\rho^\intercal \left[\mathsf{d}_{\rho\rho}\Lambda_{\rho\rho}^{-1}\mathbf{Q}_{\mathbf{t}}^{\rho}(\mathbf{t}) - \mathsf{M}_3\mathsf{R}^\intercal\mathbf{q}\right] = 0\,, \tag{S77}$$

because it involves only terms which are empty when $\rho = 0$. Similarly, the inverse MT involves an empty integral, so

$$\Upsilon_{\mathbf{t}}^{\rho}(\mathbf{q}) \doteq \int_{\mathcal{C}_0} \mathrm{d}\boldsymbol{\epsilon}_\rho\, \Psi_{\mathbf{t}}\left[\mathsf{L}\begin{pmatrix}\mathbf{Q}_{\mathbf{t}}^{\rho}(\mathbf{t}) + \boldsymbol{\epsilon}_\rho \\ \mathsf{a}_{\varsigma\varsigma}\mathbf{q}_\varsigma\end{pmatrix}\right] \exp\left[-i\gamma_{\mathbf{t}}^{\rho}(\boldsymbol{\epsilon}_\rho, \mathbf{q})\right] = \Psi_{\mathbf{t}}(\mathbf{q}_\varsigma) = \Psi_{\mathbf{t}}(q)\,. \tag{S78}$$

We next compute

$$\beta_{\mathbf{t}}^{\rho}(\mathbf{q}) \doteq \mathbf{q}^\intercal\,\mathsf{R}\mathsf{M}_4\mathsf{R}^\intercal\mathbf{q} - 2\left[\mathbf{Q}_{\mathbf{t}}^{\rho}(\mathbf{t})\right]^\intercal\,\mathsf{M}_3\mathsf{R}^\intercal\mathbf{q} + \left[\mathbf{Q}_{\mathbf{t}}^{\rho}(\mathbf{t})\right]^\intercal\,\mathsf{d}_{\rho\rho}\Lambda_{\rho\rho}^{-1}\,\mathbf{Q}_{\mathbf{t}}^{\rho}(\mathbf{t}) = 0\,. \tag{S79}$$

The inverse MT is therefore given as

$$\psi_{\mathbf{t}}(\mathbf{q}) = \frac{\sigma_{\mathbf{t}}\,\alpha_{\mathbf{t}}\exp\left[-\frac{i}{2}\beta_{\mathbf{t}}^{\rho}(\mathbf{q})\right]}{(-2\pi i)^{\rho/2}\sqrt{\det\Lambda_{\rho\rho}\det\mathsf{a}_{\varsigma\varsigma}^{-1}}}\,\Upsilon_{\mathbf{t}}^{\rho}(\mathbf{q}) = \sigma_t\alpha_t\Psi_t(q)\,. \tag{S80}$$

Finally, since there is no issue with crossing branch cuts, we can choose $\sigma_t = 1$. Thus,

$$\psi_t(q) = \alpha_0\exp(it + iq - it) = \alpha_0\exp(iq)\,. \tag{S81}$$

*9. Branch summation*

We finally must sum over branches. However, since $\tau(q)$ is single-valued, there is only one branch. Thus, we obtain

$$\psi(q) = \sum_{t\in\tau(q)}\psi_t(q) = \alpha_0\exp(iq)\,, \tag{S82}$$

which coincides with the exact result (S48).

### B. Oblique propagation in linearly stratified medium

Let us consider two-dimensional propagation in a linearly stratified medium. We align our coordinates such that the medium variation is in the $q_1$ direction, with $q_2$ homogeneous. Then, the governing equation is

$$\partial_{\mathbf{q}}^2\psi(\mathbf{q}) + (k_0^2 - q_1)\psi(\mathbf{q}) = 0\,, \tag{S83}$$

with $k_0$ a constant, or more explicitly,

$$\partial_{q_1}^2\psi(q_1, q_2) + \partial_{q_2}^2\psi(q_1, q_2) + (k_0^2 - q_1)\psi(q_1, q_2) = 0\,. \tag{S84}$$

We consider the initial conditions

$$\psi(0, q_2) = \mathrm{Ai}(0)\exp(ik_0q_2)\,. \tag{S85}$$

Note that the exact solution for these initial conditions is

$$\psi(q_1, q_2) = \mathrm{Ai}(q_1)\exp(ik_0q_2)\,. \tag{S86}$$

### 1. *Weyl symbol*

The wave equation can be equivalently written as

$$-\left[\partial_{\mathbf{q}}^2 + (k_0^2 - q_1)\right] \int \mathrm{d}\mathbf{q}'\, \delta(\mathbf{q}-\mathbf{q}')\psi(\mathbf{q}') = \int \mathrm{d}\mathbf{q}' \left[-\partial_{\mathbf{q}}^2 \delta(\mathbf{q}-\mathbf{q}') + (q_1 - k_0^2)\delta(\mathbf{q}-\mathbf{q}')\right]\psi(\mathbf{q}') = 0\,. \tag{S87}$$

Hence, the integration kernel is

$$D(\mathbf{q},\mathbf{q}') = -\partial_{\mathbf{q}-\mathbf{q}'}^2 \delta(\mathbf{q}-\mathbf{q}') + (q_1 - k_0^2)\delta(\mathbf{q}-\mathbf{q}')\,. \tag{S88}$$

We calculate the symbol as

$$\begin{aligned}\mathcal{D}(\mathbf{q},\mathbf{k}) = \int \mathrm{d}\mathbf{s}\, e^{i\mathbf{k}^\intercal \mathbf{s}} D(\mathbf{q}-\mathbf{s}/2, \mathbf{q}+\mathbf{q}/2) &= \int \mathrm{d}\mathbf{s}\, e^{i\mathbf{k}^\intercal \mathbf{s}} \left[-\partial_{-\mathbf{s}}^2 \delta(-\mathbf{s}) + (q_1 - k_0^2)\delta(-\mathbf{s})\right] \\ &= \int \mathrm{d}\mathbf{s}\, e^{-i\mathbf{k}^\intercal \mathbf{s}} \left[-\partial_{\mathbf{s}}^2 \delta(\mathbf{s}) + (q_1 - k_0^2)\delta(\mathbf{s})\right] \\ &= k_1^2 + k_2^2 + q_1 - k_0^2\,. \end{aligned} \tag{S89}$$

### 2. *Ray tracing*

The ray equations for this system are

$$\partial_{\tau_1} k_1(\boldsymbol{\tau}) = -\partial_{q_1}\mathcal{D}[\mathbf{q}(\boldsymbol{\tau}),\mathbf{k}(\boldsymbol{\tau})] = -1\,, \tag{S90a}$$
$$\partial_{\tau_1} k_2(\boldsymbol{\tau}) = -\partial_{q_2}\mathcal{D}[\mathbf{q}(\boldsymbol{\tau}),\mathbf{k}(\boldsymbol{\tau})] = 0\,, \tag{S90b}$$
$$\partial_{\tau_1} q_1(\boldsymbol{\tau}) = \partial_{k_1}\mathcal{D}[\mathbf{q}(\boldsymbol{\tau}),\mathbf{k}(\boldsymbol{\tau})] = 2k_1\,, \tag{S90c}$$
$$\partial_{\tau_1} q_2(\boldsymbol{\tau}) = \partial_{k_2}\mathcal{D}[\mathbf{q}(\boldsymbol{\tau}),\mathbf{k}(\boldsymbol{\tau})] = 2k_2\,. \tag{S90d}$$

The general solutions are

$$k_1(\boldsymbol{\tau}) = k_1(0,\tau_2) - \tau_1\,, \tag{S91a}$$
$$k_2(\boldsymbol{\tau}) = k_2(0,\tau_2)\,, \tag{S91b}$$
$$q_1(\boldsymbol{\tau}) = q_1(0,\tau_2) + 2\tau_1 k_1(0,\tau_2) - \tau_1^2\,, \tag{S91c}$$
$$q_2(\boldsymbol{\tau}) = q_2(0,\tau_2) + 2k_2(0,\tau_2)\tau_1\,. \tag{S91d}$$

Given the initial condition, it is natural to choose $q_1(0,\tau_2) = 0$. Then, the initial condition implies that $k_2(0,\tau_2) = k_0$, and our solutions become

$$k_1(\boldsymbol{\tau}) = k_1(0,\tau_2) - \tau_1\,, \tag{S92a}$$
$$k_2(\boldsymbol{\tau}) = k_0\,, \tag{S92b}$$
$$q_1(\boldsymbol{\tau}) = 2\tau_1 k_1(0,\tau_2) - \tau_1^2\,, \tag{S92c}$$
$$q_2(\boldsymbol{\tau}) = q_2(0,\tau_2) + 2k_0\tau_1\,. \tag{S92d}$$

Next, we want our initial conditions to lie on the dispersion manifold, so that the solutions always remain on the dispersion manifold. Hence, $k_1(0,\tau_2)$ is determined from the equation

$$\mathcal{D}[\mathbf{q}(0,\tau_2),\mathbf{k}(0,\tau_2)] = k_1^2(0,\tau_2) + k_0^2 - k_0^2 = 0\,. \tag{S93}$$

Clearly, this requires $k_1(0,\tau_2) = 0$. The ray solutions therefore become

$$k_1(\boldsymbol{\tau}) = -\tau_1\,, \tag{S94a}$$
$$k_2(\boldsymbol{\tau}) = k_0\,, \tag{S94b}$$
$$q_1(\boldsymbol{\tau}) = -\tau_1^2\,, \tag{S94c}$$
$$q_2(\boldsymbol{\tau}) = q_2(0,\tau_2) + 2k_0\tau_1\,. \tag{S94d}$$

Finally, since $\tau_2$ must be a parameterization of the initial conditions, it is natural to choose $q_2(0, \tau_2) = \tau_2$. Thus,

$$k_1(\boldsymbol{\tau}) = -\tau_1 \, , \tag{S95a}$$
$$k_2(\boldsymbol{\tau}) = k_0 \, , \tag{S95b}$$
$$q_1(\boldsymbol{\tau}) = -\tau_1^2 \, , \tag{S95c}$$
$$q_2(\boldsymbol{\tau}) = \tau_2 + 2k_0\tau_1 \, , \tag{S95d}$$

or in a vector form,

$$\mathbf{z}(\boldsymbol{\tau}) = \begin{pmatrix} -\tau_1^2 \\ \tau_2 + 2k_0\tau_1 \\ -\tau_1 \\ k_0 \end{pmatrix} . \tag{S96}$$

We can obtain the inverse function $\boldsymbol{\tau}(\mathbf{q})$ as

$$\tau_1(\mathbf{q}) = \pm\sqrt{-q_1} \, , \quad \tau_2(\mathbf{q}) = q_2 \mp 2k_0\sqrt{-q_1} \, . \tag{S97}$$

Clearly, $\boldsymbol{\tau}(\mathbf{q})$ is double-valued, so there will be two rays in the lit region and no rays in the shadow.

### *3. Tangent-space transformation matrix*

We perform the symplectic Gram–Schmidt algorithm to compute $\mathsf{S}_t$. Algebraically, it is easier to compute $\check{\mathbf{T}}_2(\mathbf{t})$ first, then compute $\check{\mathbf{T}}_1(\mathbf{t})$. Indeed, we first compute

$$\partial_{\tau_2}\mathbf{z}(\mathbf{t}) = \begin{pmatrix} 0 \\ 1 \\ 0 \\ 0 \end{pmatrix} . \tag{S98}$$

Thus,

$$\check{\mathbf{T}}_2(\mathbf{t}) \doteq \frac{\partial_{\tau_2}\mathbf{z}(\mathbf{t})}{\|\partial_{\tau_2}\mathbf{z}(\mathbf{t})\|} = \begin{pmatrix} 0 \\ 1 \\ 0 \\ 0 \end{pmatrix} . \tag{S99}$$

We next calculate

$$\partial_{\tau_1}\mathbf{z}(\mathbf{t}) = \begin{pmatrix} -2t_1 \\ 2k_0 \\ -1 \\ 0 \end{pmatrix} , \tag{S100}$$

and thereby compute

$$\partial_{\tau_1}\mathbf{z}(\mathbf{t}) - [\check{\mathbf{T}}_2(\mathbf{t})]^\intercal \, \partial_{\tau_1}\mathbf{z}(\mathbf{t}) = \begin{pmatrix} -2t_1 \\ 0 \\ -1 \\ 0 \end{pmatrix} . \tag{S101}$$

Thus,

$$\check{\mathbf{T}}_1(\mathbf{t}) \doteq \frac{\partial_{\tau_1}\mathbf{z}(\mathbf{t}) - [\check{\mathbf{T}}_2(\mathbf{t})]^\intercal \, \partial_{\tau_1}\mathbf{z}(\mathbf{t})}{\|\partial_{\tau_1}\mathbf{z}(\mathbf{t}) - [\check{\mathbf{T}}_2(\mathbf{t})]^\intercal \, \partial_{\tau_1}\mathbf{z}(\mathbf{t})\|} = \frac{1}{\vartheta_{\mathbf{t}}} \begin{pmatrix} -2t_1 \\ 0 \\ -1 \\ 0 \end{pmatrix} , \tag{S102}$$

where

$$\vartheta_{\mathbf{t}} \doteq \sqrt{1 + 4t_1^2} \, . \tag{S103}$$

We also compute the symplectically dual normal vectors as

$$\check{\mathbf{N}}_1(\mathbf{t}) \doteq -\mathsf{J}\,\check{\mathbf{T}}_1(\mathbf{t}) = \frac{-1}{\vartheta_{\mathbf{t}}}\begin{pmatrix} 0 & 0 & 1 & 0 \\ 0 & 0 & 0 & 1 \\ -1 & 0 & 0 & 0 \\ 0 & -1 & 0 & 0 \end{pmatrix}\begin{pmatrix} -2t_1 \\ 0 \\ -1 \\ 0 \end{pmatrix} = \frac{1}{\vartheta_{\mathbf{t}}}\begin{pmatrix} 1 \\ 0 \\ -2t_1 \\ 0 \end{pmatrix}\,, \tag{S104}$$

and similarly

$$\check{\mathbf{N}}_2(\mathbf{t}) \doteq -\mathsf{J}\,\check{\mathbf{T}}_2(\mathbf{t}) = \begin{pmatrix} 0 & 0 & -1 & 0 \\ 0 & 0 & 0 & -1 \\ 1 & 0 & 0 & 0 \\ 0 & 1 & 0 & 0 \end{pmatrix}\begin{pmatrix} 0 \\ 1 \\ 0 \\ 0 \end{pmatrix} = \begin{pmatrix} 0 \\ 0 \\ 0 \\ 1 \end{pmatrix}\,. \tag{S105}$$

Hence, we obtain

$$\mathsf{S}_{\mathbf{t}} = \begin{pmatrix} \leftarrow & \check{\mathbf{T}}_1^\intercal(\mathbf{t}) & \rightarrow \\ \leftarrow & \check{\mathbf{T}}_2^\intercal(\mathbf{t}) & \rightarrow \\ \leftarrow & \check{\mathbf{N}}_1^\intercal(\mathbf{t}) & \rightarrow \\ \leftarrow & \check{\mathbf{N}}_2^\intercal(\mathbf{t}) & \rightarrow \end{pmatrix} = \frac{1}{\vartheta_{\mathbf{t}}}\begin{pmatrix} -2t_1 & 0 & -1 & 0 \\ 0 & \vartheta_{\mathbf{t}} & 0 & 0 \\ 1 & 0 & -2t_1 & 0 \\ 0 & 0 & 0 & \vartheta_{\mathbf{t}} \end{pmatrix}\,, \tag{S106}$$

and correspondingly,

$$\mathsf{A}_{\mathbf{t}} = \mathsf{D}_{\mathbf{t}} = \frac{1}{\vartheta_{\mathbf{t}}}\begin{pmatrix} -2t_1 & 0 \\ 0 & \vartheta_{\mathbf{t}} \end{pmatrix}\,, \quad \mathsf{B}_{\mathbf{t}} = -\mathsf{C}_{\mathbf{t}} = \frac{1}{\vartheta_{\mathbf{t}}}\begin{pmatrix} -1 & 0 \\ 0 & 0 \end{pmatrix}\,. \tag{S107}$$

### *4. Tangent-space rays*

The tangent-space rays are obtained as

$$\mathbf{Q}_{\mathbf{t}}(\boldsymbol{\tau}) = \mathsf{A}_{\mathbf{t}}\,\mathbf{q}(\boldsymbol{\tau}) + \mathsf{B}_{\mathbf{t}}\,\mathbf{k}(\boldsymbol{\tau}) = \frac{1}{\vartheta_{\mathbf{t}}}\begin{pmatrix} -2t_1 & 0 \\ 0 & \vartheta_{\mathbf{t}} \end{pmatrix}\begin{pmatrix} -\tau_1^2 \\ \tau_2 + 2k_0\tau_1 \end{pmatrix} + \frac{1}{\vartheta_{\mathbf{t}}}\begin{pmatrix} -1 & 0 \\ 0 & 0 \end{pmatrix}\begin{pmatrix} -\tau_1 \\ k_0 \end{pmatrix}\,, \tag{S108}$$

$$\mathbf{K}_{\mathbf{t}}(\boldsymbol{\tau}) = \mathsf{C}_{\mathbf{t}}\,\mathbf{q}(\boldsymbol{\tau}) + \mathsf{D}_{\mathbf{t}}\,\mathbf{k}(\boldsymbol{\tau}) = \frac{1}{\vartheta_{\mathbf{t}}}\begin{pmatrix} 1 & 0 \\ 0 & 0 \end{pmatrix}\begin{pmatrix} -\tau_1^2 \\ \tau_2 + 2k_0\tau_1 \end{pmatrix} + \frac{1}{\vartheta_{\mathbf{t}}}\begin{pmatrix} -2t_1 & 0 \\ 0 & \vartheta_{\mathbf{t}} \end{pmatrix}\begin{pmatrix} -\tau_1 \\ k_0 \end{pmatrix}\,. \tag{S109}$$

Hence,

$$Q_{\mathbf{t},1}(\boldsymbol{\tau}) = \frac{2t_1\tau_1^2 + \tau_1}{\vartheta_{\mathbf{t}}}\,, \quad Q_{\mathbf{t},2}(\boldsymbol{\tau}) = \tau_2 + 2k_0\tau_1\,, \tag{S110}$$

$$K_{\mathbf{t},1}(\boldsymbol{\tau}) = \frac{2t_1\tau_1 - \tau_1^2}{\vartheta_{\mathbf{t}}}\,, \quad K_{\mathbf{t},2}(\boldsymbol{\tau}) = k_0\,. \tag{S111}$$

We also compute the inverse function $\boldsymbol{\tau}_{\mathbf{t}}(\mathbf{Q})$ as

$$\tau_{\mathbf{t},1}(\mathbf{Q}) = \frac{-1 \pm \sqrt{1 + 8t_1\vartheta_{\mathbf{t}}Q_1}}{4t_1}\,, \quad \tau_{\mathbf{t},2}(\mathbf{Q}) = Q_2 + \frac{k_0 \mp k_0\sqrt{1 + 8t_1\vartheta_{\mathbf{t}}Q_1}}{2t_1}\,. \tag{S112}$$

This allows us to construct $\mathbf{K}_{\mathbf{t}}(\mathbf{Q})$ as

$$K_{\mathbf{t},1}(\mathbf{Q}) = K_{\mathbf{t},1}[\boldsymbol{\tau}_{\mathbf{t}}(\mathbf{Q})] = \frac{-4t_1Q_1 + \vartheta_{\mathbf{t}}\left[-1 \pm \sqrt{1 + 8t_1\vartheta_{\mathbf{t}}Q_1}\right]}{8t_1^2}\,, \tag{S113}$$

$$K_{\mathbf{t},2}(\mathbf{Q}) = K_{\mathbf{t},2}[\boldsymbol{\tau}_{\mathbf{t}}(\mathbf{Q})] = k_0\,. \tag{S114}$$

The function $\mathbf{K}_{\mathbf{t}}(\mathbf{Q})$ is double-valued, but we are interested in the branch that corresponds to $\mathbf{K}_{\mathbf{t}}[\mathbf{Q}_{\mathbf{t}}(\mathbf{t})] = \mathbf{K}_{\mathbf{t}}(\mathbf{t})$.

This corresponds to the plus sign, because then,

$$\begin{aligned} K_{\mathbf{t},1}[\mathbf{Q}_{\mathbf{t}}(\mathbf{t})] &= -\frac{1}{2t_1}\frac{2t_1^3 + t_1}{\vartheta_{\mathbf{t}}} - \frac{\vartheta_{\mathbf{t}}}{8t_1^2} + \frac{\vartheta_{\mathbf{t}}}{8t_1^2}\sqrt{1 + 8t_1\vartheta_{\mathbf{t}}\frac{2t_1^3 + t_1}{\vartheta_{\mathbf{t}}}} \\ &= \frac{2t_1^2 - \vartheta_{\mathbf{t}}^2}{2\vartheta_{\mathbf{t}}} - \frac{\vartheta_{\mathbf{t}}}{8t_1^2} + \frac{\vartheta_{\mathbf{t}}}{8t_1^2}\sqrt{1 + 8t_1^2 + 16t_1^4} \\ &= \frac{2t_1^2 - \vartheta_{\mathbf{t}}^2}{2\vartheta_{\mathbf{t}}} - \frac{\vartheta_{\mathbf{t}}}{8t_1^2} + \frac{\vartheta_{\mathbf{t}}^3}{8t_1^2} \\ &= \frac{2t_1^2 - \vartheta_{\mathbf{t}}^2}{2\vartheta_{\mathbf{t}}} + \frac{\vartheta_{\mathbf{t}}}{2} \\ &= \frac{t_1^2}{\vartheta_{\mathbf{t}}} \\ &= K_{\mathbf{t}}(\mathbf{t})\,. \end{aligned} \tag{S115}$$

Then, in summary:

$$K_{\mathbf{t},1}(\mathbf{Q}) = \frac{-4t_1Q_1 + \vartheta_{\mathbf{t}}\left[-1 + \sqrt{1 + 8t_1\vartheta_{\mathbf{t}}Q_1}\right]}{8t_1^2}\,, \quad K_{\mathbf{t},2}(\mathbf{Q}) = k_0\,. \tag{S116}$$

### *5. Tangent-space phase*

Consider the wave phase on the tangent space

$$\Theta_{\mathbf{t}}(\mathbf{Q}) = \int_{\mathbf{Q}_{\mathbf{t}}(\mathbf{t})}^{\mathbf{Q}} \left[\mathbf{K}_{\mathbf{t}}(\mathbf{Q}')\right]^{\intercal} \mathrm{d}\mathbf{Q}' = \int_{Q_{\mathbf{t},1}(\mathbf{t})}^{Q_1} \mathrm{d}Q_1'\, K_{\mathbf{t},1}[Q_1', Q_{\mathbf{t},2}(\mathbf{t})] + \int_{Q_{\mathbf{t},2}(\mathbf{t})}^{Q_2} \mathrm{d}Q_2'\, K_{\mathbf{t},2}(Q_1, Q_2')\,, \tag{S117}$$

where we have chosen the integration contour to be the union of two straight line paths. Then, we compute

$$\begin{aligned} \Theta_{\mathbf{t}}(\mathbf{Q}) &= \int_{Q_{\mathbf{t},1}(\mathbf{t})}^{Q_1} \mathrm{d}Q_1'\, \frac{-4t_1Q_1 + \vartheta_{\mathbf{t}}\left[-1 + \sqrt{1 + 8t_1\vartheta_{\mathbf{t}}Q_1}\right]}{8t_1^2} + \int_{Q_{\mathbf{t},2}(\mathbf{t})}^{Q_2} \mathrm{d}Q_2'\, k_0 \\ &= \frac{Q_{\mathbf{t},1}^2(\mathbf{t}) - Q_1^2}{4t_1} + \frac{\vartheta_{\mathbf{t}}\left[Q_{\mathbf{t},1}(\mathbf{t}) - Q_1\right]}{8t_1^2} + \frac{(1 + 8t_1\vartheta_{\mathbf{t}}Q_1)^{3/2} - [1 + 8t_1\vartheta_{\mathbf{t}}Q_{\mathbf{t},1}(\mathbf{t})]^{3/2}}{96t_1^3} + k_0\left[Q_2 - Q_{\mathbf{t},2}(\mathbf{t})\right]. \end{aligned} \tag{S118}$$

Let us introduce $\boldsymbol{\epsilon} \doteq \mathbf{Q} - \mathbf{Q}_{\mathbf{t}}(\mathbf{t})$. Then, $\Theta(\mathbf{Q}) \equiv \Theta[\mathbf{Q}_{\mathbf{t}}(\mathbf{t}) + \boldsymbol{\epsilon}]$ is given by

$$\begin{aligned} \Theta_{\mathbf{t}}[\boldsymbol{\epsilon} + \mathbf{Q}_{\mathbf{t}}(\mathbf{t})] &= -\frac{\epsilon_1^2}{4t_1} - \frac{4t_1Q_{\mathbf{t},1}(\mathbf{t}) + \vartheta_{\mathbf{t}}}{8t_1^2}\epsilon_1 + \frac{[1 + 8t_1\vartheta_{\mathbf{t}}Q_{\mathbf{t},1}(\mathbf{t}) + 8t_1\vartheta_{\mathbf{t}}\epsilon_1]^{3/2} - [1 + 8t_1\vartheta_{\mathbf{t}}Q_{\mathbf{t},1}(\mathbf{t})]^{3/2}}{96t_1^3} + k_0\epsilon_2 \\ &= -\frac{\epsilon_1^2}{4t_1} + \frac{8t_1^4 - \vartheta_{\mathbf{t}}^4}{8t_1^2\vartheta_{\mathbf{t}}}\epsilon_1 + \frac{\left(\vartheta_{\mathbf{t}}^4 + 8t_1\vartheta_{\mathbf{t}}\epsilon_1\right)^{3/2} - \vartheta_{\mathbf{t}}^6}{96t_1^3} + k_0\epsilon_2\,. \end{aligned} \tag{S119}$$

### *6. Tangent-space envelope*

We compute

$$J_{\mathbf{t}}(\boldsymbol{\tau}) \doteq \det \partial_{\boldsymbol{\tau}}\mathbf{Q}_{\mathbf{t}}(\boldsymbol{\tau}) = \det\begin{vmatrix} \partial_{\tau_1}Q_{\mathbf{t},1}(\boldsymbol{\tau}) & \partial_{\tau_1}Q_{\mathbf{t},2}(\boldsymbol{\tau}) \\ \partial_{\tau_2}Q_{\mathbf{t},1}(\boldsymbol{\tau}) & \partial_{\tau_2}Q_{\mathbf{t},2}(\boldsymbol{\tau}) \end{vmatrix} = \det\begin{vmatrix} \frac{4t_1\tau_1+1}{\vartheta_{\mathbf{t}}} & 2k_0 \\ 0 & 1 \end{vmatrix} = \frac{4t_1\tau_1 + 1}{\vartheta_{\mathbf{t}}}\,. \tag{S120}$$

Therefore, $J_{\mathbf{t}}(t_1, \boldsymbol{\tau}_\perp) = \vartheta_{\mathbf{t}}$, and Eq. (27) of the main text leads to

$$\Phi_{\mathbf{t}}\left[\mathbf{Q}_{\mathbf{t}}(\boldsymbol{\tau})\right] = \Phi_{\mathbf{t}}\left[\mathbf{Q}_{\mathbf{t}}(t_1, \boldsymbol{\tau}_\perp)\right]\frac{\vartheta_{\mathbf{t}}}{\sqrt{4t_1\tau_1 + 1}}\,. \tag{S121}$$

For simplicity, let us assume the initial conditions such that $\Phi_{\mathbf{t}}\left[\mathbf{Q}_{\mathbf{t}}(t_1, \boldsymbol{\tau}_\perp)\right] = 1$. Then,

$$\Phi_{\mathbf{t}}\left[\mathbf{Q}_{\mathbf{t}}(\boldsymbol{\tau})\right] = \frac{\vartheta_{\mathbf{t}}}{\sqrt{4t_1\tau_1 + 1}} \, . \tag{S122}$$

Lastly, we must insert $\tau_{\mathbf{t},1}(\mathbf{Q})$ to obtain $\Phi_{\mathbf{t}}\left[\mathbf{Q}_{\mathbf{t}}(\boldsymbol{\tau})\right]$:

$$\Phi_{\mathbf{t}}(\mathbf{Q}) = \frac{\vartheta_{\mathbf{t}}}{\sqrt{4t_1 \frac{-1+\sqrt{1+8t_1\vartheta_{\mathbf{t}}Q_1}}{4t_1} + 1}} = \frac{\vartheta_{\mathbf{t}}}{\left(1 + 8t_1\vartheta_{\mathbf{t}}Q_1\right)^{1/4}} \, . \tag{S123}$$

In terms of $\boldsymbol{\epsilon}$, this reads

$$\Phi_{\mathbf{t}}\left[\boldsymbol{\epsilon} + \mathbf{Q}_{\mathbf{t}}(\mathbf{t})\right] = \frac{\vartheta_{\mathbf{t}}}{\left[1 + 8t_1\vartheta_{\mathbf{t}}Q_{\mathbf{t},1}(\mathbf{t}) + 8t_1\vartheta_{\mathbf{t}}\epsilon_1\right]^{1/4}} = \frac{\vartheta_{\mathbf{t}}}{\left(\vartheta_{\mathbf{t}}^4 + 8t_1\vartheta_{\mathbf{t}}\epsilon_1\right)^{1/4}} \, . \tag{S124}$$

### 7. *Linking with NIMT*

We compute

$$\mathsf{S}_{\mathbf{t}}^{-1} = \begin{pmatrix} \mathsf{D}^\intercal & -\mathsf{B}^\intercal \\ -\mathsf{C}^\intercal & \mathsf{A}^\intercal \end{pmatrix} = \frac{1}{\vartheta_{\mathbf{t}}} \begin{pmatrix} -2t_1 & 0 & 1 & 0 \\ 0 & \vartheta_{\mathbf{t}} & 0 & 0 \\ -1 & 0 & -2t_1 & 0 \\ 0 & 0 & 0 & \vartheta_{\mathbf{t}} \end{pmatrix} \tag{S125}$$

and also

$$\partial_{t_1}\mathsf{S}_{\mathbf{t}} = \partial_{t_1} \begin{pmatrix} \frac{-2t_1}{\sqrt{4t_1^2+1}} & 0 & \frac{-1}{\sqrt{4t_1^2+1}} & 0 \\ 0 & 1 & 0 & 0 \\ \frac{1}{\sqrt{4t_1^2+1}} & 0 & \frac{-2t_1}{\sqrt{4t_1^2+1}} & 0 \\ 0 & 0 & 0 & 1 \end{pmatrix} = \frac{1}{\vartheta_{\mathbf{t}}^3} \begin{pmatrix} -2 & 0 & 4t_1 & 0 \\ 0 & 0 & 0 & 0 \\ -4t_1 & 0 & -2 & 0 \\ 0 & 0 & 0 & 0 \end{pmatrix} \, . \tag{S126}$$

Therefore, we compute

$$\left(\partial_{t_1}\mathsf{S}_{\mathbf{t}}\right)\mathsf{S}_{\mathbf{t}}^{-1} = \frac{1}{\vartheta_{\mathbf{t}}^4} \begin{pmatrix} -2 & 0 & 4t_1 & 0 \\ 0 & 0 & 0 & 0 \\ -4t_1 & 0 & -2 & 0 \\ 0 & 0 & 0 & 0 \end{pmatrix} \begin{pmatrix} -2t_1 & 0 & 1 & 0 \\ 0 & \vartheta_{\mathbf{t}} & 0 & 0 \\ -1 & 0 & -2t_1 & 0 \\ 0 & 0 & 0 & \vartheta_{\mathbf{t}} \end{pmatrix} = \frac{2}{\vartheta_{\mathbf{t}}^2} \begin{pmatrix} 0 & 0 & -1 & 0 \\ 0 & 0 & 0 & 0 \\ 1 & 0 & 0 & 0 \\ 0 & 0 & 0 & 0 \end{pmatrix} \tag{S127}$$

and consequently identify

$$\mathsf{V}_{\mathbf{t}} = \mathsf{0}_2 \, , \quad \mathsf{U}_{\mathbf{t}} = \mathsf{W}_{\mathbf{t}} = \begin{pmatrix} -\frac{2}{\vartheta_{\mathbf{t}}^2} & 0 \\ 0 & 0 \end{pmatrix} \, . \tag{S128}$$

We also compute

$$\partial_{t_1}\mathbf{Q}_{\mathbf{t}}(\mathbf{t}) = \partial_{t_1} \begin{pmatrix} \frac{2t_1^3+t_1}{\vartheta_{\mathbf{t}}} \\ t_2 + 2k_0t_1 \end{pmatrix} = \begin{pmatrix} \frac{\vartheta^4(\mathbf{t})-2t_1^2}{\vartheta_{\mathbf{t}}^3} \\ 2k_0 \end{pmatrix} \tag{S129}$$

and

$$\partial_{\mathbf{Q}}\Phi_{\mathbf{t}}(\mathbf{Q}) = \begin{pmatrix} \partial_{Q_1}\Phi_{\mathbf{t}}(\mathbf{Q}) \\ \partial_{Q_2}\Phi_{\mathbf{t}}(\mathbf{Q}) \end{pmatrix} = \begin{pmatrix} -\frac{2\vartheta_{\mathbf{t}}^2 t_1}{(\vartheta_{\mathbf{t}}^4+8t_1\vartheta_{\mathbf{t}}\epsilon_1)^{5/4}} \\ 0 \end{pmatrix} \, , \tag{S130}$$

which implies that

$$\partial_{\mathbf{Q}}\Phi_{\mathbf{t}}\left[\mathbf{Q}_{\mathbf{t}}(\mathbf{t})\right] = \begin{pmatrix} -\frac{2t_1}{\vartheta_{\mathbf{t}}^3} \\ 0 \end{pmatrix} \, . \tag{S131}$$

Therefore,

$$
\begin{aligned}
\eta_{\mathbf{t}} &\doteq \left[\partial_{t_1}\mathbf{Q}_{\mathbf{t}}(\mathbf{t}) - \mathsf{V}_{\mathbf{t}}^\intercal \mathbf{Q}_{\mathbf{t}}(\mathbf{t})\right]^\intercal \left\{\partial_{\mathbf{Q}}\Phi_{\mathbf{t}}\left[\mathbf{Q}_{\mathbf{t}}(\mathbf{t})\right] + i\mathbf{K}_{\mathbf{t}}(\mathbf{t})\right\} \\
&\quad - \mathbf{K}_{\mathbf{t}}^\intercal(\mathbf{t})\mathsf{W}_{\mathbf{t}}\left\{\partial_{\mathbf{Q}}\Phi_{\mathbf{t}}\left[\mathbf{Q}_{\mathbf{t}}(\mathbf{t})\right] + \frac{i}{2}\mathbf{K}_{\mathbf{t}}(\mathbf{t})\right\} - \frac{1}{2}\mathrm{tr}\left(\mathsf{V}_{\mathbf{t}}\right) - \frac{i}{2}\mathbf{Q}_{\mathbf{t}}^\intercal(\mathbf{t})\mathsf{U}_{\mathbf{t}}\mathbf{Q}_{\mathbf{t}}(\mathbf{t}) \\
&= \begin{pmatrix}\frac{\vartheta_{\mathbf{t}}^4 - 2t_1^2}{\vartheta_{\mathbf{t}}^3} & 2k_0\end{pmatrix}\begin{pmatrix}-\frac{2t_1}{\vartheta_{\mathbf{t}}^3} + i\frac{t_1^2}{\vartheta_{\mathbf{t}}} \\ ik_0\end{pmatrix} - \begin{pmatrix}\frac{t_1^2}{\vartheta_{\mathbf{t}}} & k_0\end{pmatrix}\begin{pmatrix}-\frac{2}{\vartheta_{\mathbf{t}}^2} & 0 \\ 0 & 0\end{pmatrix}\begin{pmatrix}-\frac{2t_1}{\vartheta_{\mathbf{t}}^3} + \frac{i}{2}\frac{t_1^2}{\vartheta_{\mathbf{t}}} \\ \frac{i}{2}k_0\end{pmatrix} \\
&\quad - \frac{i}{2}\begin{pmatrix}\frac{t_1 + 2t_1^3}{\vartheta_{\mathbf{t}}} & t_2 + 2k_0 t_1\end{pmatrix}\begin{pmatrix}-\frac{2}{\vartheta_{\mathbf{t}}^2} & 0 \\ 0 & 0\end{pmatrix}\begin{pmatrix}\frac{t_1 + 2t_1^3}{\vartheta_{\mathbf{t}}} \\ t_2 + 2k_0 t_1\end{pmatrix} \\
&= \begin{pmatrix}\frac{\vartheta_{\mathbf{t}}^4 - 2t_1^2}{\vartheta_{\mathbf{t}}^3} & 2k_0\end{pmatrix}\begin{pmatrix}-\frac{2t_1}{\vartheta_{\mathbf{t}}^3} + i\frac{t_1^2}{\vartheta_{\mathbf{t}}} \\ ik_0\end{pmatrix} + \begin{pmatrix}\frac{2t_1^2}{\vartheta_{\mathbf{t}}^3} & 0\end{pmatrix}\begin{pmatrix}-\frac{2t_1}{\vartheta_{\mathbf{t}}^3} + \frac{i}{2}\frac{t_1^2}{\vartheta_{\mathbf{t}}} \\ \frac{i}{2}k_0\end{pmatrix} + i\begin{pmatrix}\frac{t_1 + 2t_1^3}{\vartheta_{\mathbf{t}}^3} & 0\end{pmatrix}\begin{pmatrix}\frac{t_1 + 2t_1^3}{\vartheta_{\mathbf{t}}} \\ t_2 + 2k_0 t_1\end{pmatrix}. \\
&= \frac{-2t_1\vartheta_{\mathbf{t}}^4 + 4t_1^3 - 4t_1^3}{\vartheta_{\mathbf{t}}^6} + i\frac{t_1^2\vartheta_{\mathbf{t}}^4 - 2t_1^4 + t_1^4 + (t_1 + 2t_1^3)^2}{\vartheta_{\mathbf{t}}^4} + 2ik_0^2 \\
&= -\frac{2t_1}{\vartheta_{\mathbf{t}}^2} + i\frac{20t_1^6 + 11t_1^4 + 2t_1^2}{\vartheta_{\mathbf{t}}^4} + 2ik_0^2\,.
\end{aligned}
\tag{S132}
$$

Hence, $\alpha_{\mathbf{t}}$ is computed as

$$
\begin{aligned}
\alpha_{\mathbf{t}} = \alpha_{(0,t_2)}\exp\left[\int_0^{t_1}\mathrm{d}h\,\eta_{(h,t_2)}\right] &= \alpha_{(0,t_2)}\exp\left\{\int_0^{t_1}\mathrm{d}h\,\left[-\frac{2h}{4h^2+1} + i\frac{20h^6 + 11h^4 + 2h^2}{(4h^2+1)^2} + 2ik_0^2\right]\right\} \\
&= \alpha_{(0,t_2)}\exp\left(-\frac{1}{2}\log\vartheta_{\mathbf{t}} + i\frac{2t_1^3}{3} - i\frac{t_1^5}{\vartheta_{\mathbf{t}}^2} + 2ik_0^2 t_1\right) \\
&= \frac{\alpha_{(0,t_2)}}{\sqrt{\vartheta_{\mathbf{t}}}}\exp\left(2ik_0^2 t_1 + i\frac{2t_1^3}{3} - i\frac{t_1^5}{\vartheta_{\mathbf{t}}^2}\right)\,,
\end{aligned}
\tag{S133}
$$

where $\alpha_{(0,t_2)}$ is an arbitrary function determined by initial conditions.

### 8. *Inverse MT*

Note that $\mathsf{B}$ is already in the desired SVD form. We therefore identify the submatrices

$$\Lambda_{\rho\rho} = -\frac{1}{\vartheta_{\mathbf{t}}}\,, \tag{S134}$$

$$\mathsf{a}_{\rho\rho} = -\frac{2t_1}{\vartheta_{\mathbf{t}}}\,, \quad \mathsf{a}_{\rho\varsigma} = 0\,, \quad \mathsf{a}_{\varsigma\varsigma} = 1\,, \tag{S135}$$

$$\mathsf{c}_{\rho\rho} = \frac{1}{\vartheta_{\mathbf{t}}}\,, \quad \mathsf{c}_{\rho\varsigma} = 0\,, \quad \mathsf{c}_{\varsigma\rho} = 0\,, \quad \mathsf{c}_{\varsigma\varsigma} = 0\,, \tag{S136}$$

$$\mathsf{d}_{\rho\rho} = -\frac{2t_1}{\vartheta_{\mathbf{t}}}\,, \quad \mathsf{d}_{\varsigma\rho} = 0\,, \quad \mathsf{d}_{\varsigma\varsigma} = 1\,. \tag{S137}$$

We can also construct the matrices

$$\mathsf{L} = \mathsf{I}_2\,, \tag{S138}$$

$$\mathsf{R} = \mathsf{I}_2\,, \tag{S139}$$

$$\mathsf{M}_3 \doteq \begin{pmatrix}\Lambda_{\rho\rho}^{-1} & -\Lambda_{\rho\rho}^{-1}\mathsf{d}_{\varsigma\rho}^\intercal\mathsf{a}_{\varsigma\varsigma}\end{pmatrix} = \begin{pmatrix}-\vartheta_{\mathbf{t}} & 0\end{pmatrix}\,, \tag{S140}$$

$$\mathsf{M}_4 \doteq \begin{pmatrix}\Lambda_{\rho\rho}^{-1}\mathsf{a}_{\rho\rho} & \Lambda_{\rho\rho}^{-1}\mathsf{a}_{\rho\varsigma} \\ \mathsf{a}_{\rho\varsigma}^\intercal\Lambda_{\rho\rho}^{-1} & \mathsf{a}_{\varsigma\varsigma}^\intercal\mathsf{c}_{\varsigma\varsigma} - \mathsf{a}_{\varsigma\varsigma}^\intercal\mathsf{d}_{\varsigma\rho}\Lambda_{\rho\rho}^{-1}\mathsf{a}_{\rho\varsigma}\end{pmatrix} = \begin{pmatrix}2t_1 & 0 \\ 0 & 0\end{pmatrix}\,. \tag{S141}$$

Then, since $\boldsymbol{\epsilon}_\rho = \epsilon_1$ and $\mathbf{Q}^\rho_{\mathbf{t}}(\mathbf{t}) = Q_{\mathbf{t},1}(\mathbf{t})$, we calculate

$$\begin{aligned}
\beta^\rho_{\mathbf{t}}(\mathbf{q}) &\doteq \mathbf{q}^\intercal\, \mathsf{R}\mathsf{M}_4\mathsf{R}^\intercal \mathbf{q} - 2\left[\mathbf{Q}^\rho_{\mathbf{t}}(\mathbf{t})\right]^\intercal\, \mathsf{M}_3\mathsf{R}^\intercal\mathbf{q} + \left[\mathbf{Q}^\rho_{\mathbf{t}}(\mathbf{t})\right]^\intercal\, \mathsf{d}_{\rho\rho}\Lambda^{-1}_{\rho\rho}\, \mathbf{Q}^\rho_{\mathbf{t}}(\mathbf{t}) \\
&= \begin{pmatrix} q_1 & q_2 \end{pmatrix} \begin{pmatrix} 2t_1 & 0 \\ 0 & 0 \end{pmatrix} \begin{pmatrix} q_1 \\ q_2 \end{pmatrix} - 2Q_{\mathbf{t},1}(\mathbf{t}) \begin{pmatrix} -\vartheta_{\mathbf{t}} & 0 \end{pmatrix} \begin{pmatrix} q_1 \\ q_2 \end{pmatrix} + 2t_1[Q_{\mathbf{t},1}(\mathbf{t})]^2 \\
&= 2t_1 q_1^2 + 2\vartheta_{\mathbf{t}} Q_{\mathbf{t},1}(\mathbf{t}) q_1 + 2t_1[Q_{\mathbf{t},1}(\mathbf{t})]^2 \\
&= 2t_1 q_1^2 + (4t_1^3 + 2t_1)q_1 + \frac{8t_1^7 + 8t_1^5 + 2t_1^3}{4t_1^2+1} \, .
\end{aligned} \tag{S142}$$

When evaluated at $q_1 = q_1(\mathbf{t}) = -t_1^2$, this becomes

$$\beta^\rho_{\mathbf{t}}[\mathbf{q}(\mathbf{t})] = -\frac{2t_1^5}{\vartheta_{\mathbf{t}}^2} \, . \tag{S143}$$

We also compute

$$\begin{aligned}
\gamma^\rho_{\mathbf{t}}(\boldsymbol{\epsilon}_\rho, \mathbf{q}) &\doteq \frac{1}{2}\boldsymbol{\epsilon}_\rho^\intercal\, \mathsf{d}_{\rho\rho}\Lambda^{-1}_{\rho\rho}\, \boldsymbol{\epsilon}_\rho + \boldsymbol{\epsilon}_\rho^\intercal \left[\mathsf{d}_{\rho\rho}\Lambda^{-1}_{\rho\rho}\mathbf{Q}^\rho_{\mathbf{t}}(\mathbf{t}) - \mathsf{M}_3\mathsf{R}^\intercal\mathbf{q}\right] \\
&= t_1\epsilon_1^2 + \epsilon_1[2t_1 Q_{\mathbf{t},1}(\mathbf{t}) + \vartheta_{\mathbf{t}} q_1] \\
&= t_1\epsilon_1^2 + \frac{2t_1^2 + 4t_1^4 + (4t_1^2+1)q_1}{\vartheta_{\mathbf{t}}}\epsilon_1 \, .
\end{aligned} \tag{S144}$$

When evaluated at $q_1 = q_1(\mathbf{t}) = -t_1^2$, this becomes

$$\gamma^\rho_{\mathbf{t}}[\boldsymbol{\epsilon}_\rho, \mathbf{q}(\mathbf{t})] = t_1\epsilon_1^2 + \frac{t_1^2}{\vartheta_{\mathbf{t}}}\epsilon_1 \, . \tag{S145}$$

Next, since $\mathbf{q}_\varsigma = q_2$, we compute

$$\begin{aligned}
\Upsilon^\rho_{\mathbf{t}}(\mathbf{q}) &\doteq \int_{\mathcal{C}_0} \mathrm{d}\boldsymbol{\epsilon}_\rho\, \Psi_{\mathbf{t}}\left[\mathsf{L}\begin{pmatrix} \mathbf{Q}^\rho_{\mathbf{t}}(\mathbf{t}) + \boldsymbol{\epsilon}_\rho \\ \mathsf{a}_{\varsigma\varsigma}\mathbf{q}_\varsigma \end{pmatrix}\right] \exp\left[-i\gamma^\rho_{\mathbf{t}}(\boldsymbol{\epsilon}_\rho, \mathbf{q})\right] \\
&= \int_{\mathcal{C}_0} \mathrm{d}\epsilon_1\, \Psi_{\mathbf{t}}\left[Q_{\mathbf{t},1}(\mathbf{t}) + \epsilon_1, q_2\right] \exp\left[-i\gamma^\rho_{\mathbf{t}}(\boldsymbol{\epsilon}_\rho, \mathbf{q})\right] \\
&= \int_{\mathcal{C}_0} \mathrm{d}\epsilon_1\, \frac{\vartheta_{\mathbf{t}}}{\left(\vartheta_{\mathbf{t}}^4 + 8t_1\vartheta_{\mathbf{t}}\epsilon_1\right)^{1/4}} \\
&\quad \times \exp\left\{-i\frac{\epsilon_1^2}{4t_1} + i\frac{8t_1^4 - \vartheta_{\mathbf{t}}^4}{8t_1^2\vartheta_{\mathbf{t}}}\epsilon_1 + i\frac{\left(\vartheta_{\mathbf{t}}^4 + 8t_1\vartheta_{\mathbf{t}}\epsilon_1\right)^{3/2} - \vartheta_{\mathbf{t}}^6}{96t_1^3} + ik_0[q_2 - Q_{\mathbf{t},2}(\mathbf{t})] - i\gamma^\rho_{\mathbf{t}}(\boldsymbol{\epsilon}_\rho, \mathbf{q})\right\} \\
&= \int_{\mathcal{C}_0} \mathrm{d}\epsilon_1\, \frac{\vartheta_{\mathbf{t}}}{\left(\vartheta_{\mathbf{t}}^4 + 8t_1\vartheta_{\mathbf{t}}\epsilon_1\right)^{1/4}} \\
&\quad \times \exp\left[-i\frac{\epsilon_1^2}{4t_1} + i\frac{8t_1^4 - \vartheta_{\mathbf{t}}^4}{8t_1^2\vartheta_{\mathbf{t}}}\epsilon_1 + i\frac{\left(\vartheta_{\mathbf{t}}^4 + 8t_1\vartheta_{\mathbf{t}}\epsilon_1\right)^{3/2} - \vartheta_{\mathbf{t}}^6}{96t_1^3} + ik_0q_2 - ik_0t_2 - 2ik_0^2t_1 - i\gamma^\rho_{\mathbf{t}}(\boldsymbol{\epsilon}_\rho, \mathbf{q})\right] \, .
\end{aligned} \tag{S146}$$

When evaluated at $\mathbf{q} = \mathbf{q}(\mathbf{t})$, this becomes

$$\Upsilon^\rho_{\mathbf{t}}\left[\mathbf{q}(\mathbf{t})\right] = \int_{\mathcal{C}_0} \mathrm{d}\epsilon_1\, \frac{\vartheta_{\mathbf{t}}}{\left(\vartheta_{\mathbf{t}}^4 + 8t_1\vartheta_{\mathbf{t}}\epsilon_1\right)^{1/4}} \exp\left[-i\frac{\vartheta_{\mathbf{t}}^2}{4t_1}\epsilon_1^2 - i\frac{\vartheta_{\mathbf{t}}^3}{8t_1^2}\epsilon_1 + i\frac{\left(\vartheta_{\mathbf{t}}^4 + 8t_1\vartheta_{\mathbf{t}}\epsilon_1\right)^{3/2} - \vartheta_{\mathbf{t}}^6}{96t_1^3}\right] \, . \tag{S147}$$

This is the exact same integral that was studied in Ref. [3]. Indeed, upon expanding around $\epsilon_1 = 0$ we obtain Eq. (113) of Ref. [3], namely,

$$\Upsilon^\rho_{\mathbf{t}}\left[\mathbf{q}(\mathbf{t})\right] \approx \int_{\mathcal{C}_0} \mathrm{d}\epsilon_1\, \exp\left(-it_1\epsilon_1^2 - i\frac{\epsilon_1^3}{3\vartheta_{\mathbf{t}}^3}\right) \, . \tag{S148}$$

Therefore, we immediately conclude that

$$\Upsilon^{\rho}_{\mathbf{t}}\left[\mathbf{q}(\mathbf{t})\right] \approx \pi \vartheta_{\mathbf{t}} \exp\left(-i\frac{2}{3}t_1^3 \vartheta_{\mathbf{t}}^6\right)\left[\mathrm{Ai}(-t_1^2\vartheta_{\mathbf{t}}^4) - i\,\mathrm{sign}(t_1)\mathrm{Bi}(-t_1^2\vartheta_{\mathbf{t}}^4)\right] \, . \tag{S149}$$

Putting everything together, we obtain

$$\begin{aligned}
\psi_{\mathbf{t}}[\mathbf{q}(\mathbf{t})] &= \frac{\sigma_{\mathbf{t}}\, \alpha_{\mathbf{t}} \exp\left\{-\frac{i}{2}\beta^{\rho}_{\mathbf{t}}[\mathbf{q}(\mathbf{t})]\right\}}{(-2\pi i)^{\rho/2}\sqrt{\det \Lambda_{\rho\rho} \det \mathsf{a}^{-1}_{\varsigma\varsigma}}}\, \Upsilon^{\rho}_{\mathbf{t}}[\mathbf{q}(\mathbf{t})] \\
&= \frac{\sigma_{\mathbf{t}}\, \alpha_{\mathbf{t}} \exp\left(i\frac{t_1^5}{\vartheta_{\mathbf{t}}^2}\right)}{\sqrt{-2\pi i}\sqrt{-\frac{1}{\vartheta_{\mathbf{t}}}}}\, \pi\vartheta_{\mathbf{t}} \exp\left(-i\frac{2}{3}t_1^3\vartheta_{\mathbf{t}}^6\right)\left[\mathrm{Ai}(-t_1^2\vartheta_{\mathbf{t}}^4) - i\,\mathrm{sign}(t_1)\mathrm{Bi}(-t_1^2\vartheta_{\mathbf{t}}^4)\right] \\
&= \frac{\sigma_{\mathbf{t}}\, \pi\vartheta_{\mathbf{t}}}{\sqrt{-2\pi i}\sqrt{-\frac{1}{\vartheta_{\mathbf{t}}}}}\, \frac{\alpha_{(0,t_2)}}{\sqrt{\vartheta_{\mathbf{t}}}} \exp\left[2ik_0^2 t_1 + i\frac{2t_1^3}{3}\left(1-\vartheta_{\mathbf{t}}^6\right)\right]\left[\mathrm{Ai}(-t_1^2\vartheta_{\mathbf{t}}^4) - i\,\mathrm{sign}(t_1)\mathrm{Bi}(-t_1^2\vartheta_{\mathbf{t}}^4)\right] \\
&= \frac{\sigma_{\mathbf{t}}\, \pi\vartheta_{\mathbf{t}}\alpha_{(0,t_2)}}{\sqrt{-2\pi i}\sqrt{-1}} \exp\left[2ik_0^2 t_1 + i\frac{2t_1^3}{3}\left(1-\vartheta_{\mathbf{t}}^6\right)\right]\left[\mathrm{Ai}(-t_1^2\vartheta_{\mathbf{t}}^4) - i\,\mathrm{sign}(t_1)\mathrm{Bi}(-t_1^2\vartheta_{\mathbf{t}}^4)\right] \, .
\end{aligned} \tag{S150}$$

Since there are no issues with crossing the branch cut, we can set $\sigma_{\mathbf{t}} = 1$. Then, since our branch-cut convention dictates $1/\sqrt{-1} = \exp(i\pi/2) = i$, we obtain

$$\psi_{\mathbf{t}}[\mathbf{q}(\mathbf{t})] = i\alpha_{(0,t_2)}\frac{\sqrt{\pi}}{\sqrt{-2i}}\vartheta_{\mathbf{t}} \exp\left[2ik_0^2 t_1 + i\frac{2t_1^3}{3}\left(1-\vartheta_{\mathbf{t}}^6\right)\right]\left[\mathrm{Ai}(-t_1^2\vartheta_{\mathbf{t}}^4) - i\,\mathrm{sign}(t_1)\mathrm{Bi}(-t_1^2\vartheta_{\mathbf{t}}^4)\right] \, . \tag{S151}$$

### *9. Branch summation*

We must sum over both branches, given as $t_1 = \sqrt{-q_1}, t_2 = q_2 - 2k_0\sqrt{-q_1}$ and $t_1 = -\sqrt{-q_1}, t_2 = q_2 + 2k_0\sqrt{-q_1}$. Therefore,

$$\begin{aligned}
\psi(\mathbf{q}) &= \sum_{\mathbf{t}\in\boldsymbol{\tau}(\mathbf{q})} \psi_{\mathbf{t}}[\mathbf{q}(\mathbf{t})] \\
&= i\alpha_{(0,q_2-2k_0\sqrt{-q_1})}\frac{\sqrt{\pi}}{\sqrt{-2i}}\sqrt{1-4q_1^2}\, \exp\left\{2ik_0^2\sqrt{-q_1} + i\frac{2}{3}(-q_1)^{3/2}\left[1-(1-4q_1)^3\right]\right\} \\
&\qquad\qquad \times \left\{\mathrm{Ai}[q_1(1-4q_1)^2] - i\,\mathrm{Bi}[q_1(1-4q_1)^2]\right\} \\
&\quad + i\alpha_{(0,q_2+2k_0\sqrt{-q_1})}\frac{\sqrt{\pi}}{\sqrt{-2i}}\sqrt{1-4q_1^2}\, \exp\left\{-2ik_0^2\sqrt{-q_1} - i\frac{2}{3}(-q_1)^{3/2}\left[1-(1-4q_1)^3\right]\right\} \\
&\qquad\qquad \times \left\{\mathrm{Ai}[q_1(1-4q_1)^2] + i\,\mathrm{Bi}[q_1(1-4q_1)^2]\right\} \, .
\end{aligned} \tag{S152}$$

To match the initial condition $\psi(0,q_2) = \mathrm{Ai}(0)\exp(ik_0 q_2)$, we must choose

$$\alpha_{(0,t_2)} = \frac{\sqrt{-2i}}{2i\sqrt{\pi}}\exp(ik_0 t_2)\, . \tag{S153}$$

Then, $\psi(\mathbf{q})$ becomes

$$\begin{aligned}
\psi(\mathbf{q}) &= \frac{\sqrt{1-4q_1^2}\exp(ik_0q_2)}{2}\exp\left[-i\varpi(q_1)\right]\left\{\mathrm{Ai}[-\varrho^2(q_1)] - i\,\mathrm{Bi}[-\varrho^2(q_1)]\right\} \\
&\quad + \frac{\sqrt{1-4q_1^2}\exp(ik_0q_2)}{2}\exp\left[i\varpi(q_1)\right]\left\{\mathrm{Ai}[-\varrho^2(q_1)] + i\,\mathrm{Bi}[-\varrho^2(q_1)]\right\} \\
&= \frac{\sqrt{1-4q_1^2}\exp(ik_0q_2)}{2}\mathrm{Ai}[-\varrho^2(q_1)]\left\{\exp\left[i\varpi(q_1)\right] + \exp\left[-i\varpi(q_1)\right]\right\} \\
&\quad + i\frac{\sqrt{1-4q_1^2}\exp(ik_0q_2)}{2}\mathrm{Bi}[-\varrho^2(q_1)]\left\{\exp\left[i\varpi(q_1)\right] - \exp\left[-i\varpi(q_1)\right]\right\} \\
&= \sqrt{1-4q_1}\exp(ik_0q_2)\left\{\mathrm{Ai}[-\varrho^2(q_1)]\cos\varpi(q_1) - \mathrm{Bi}[-\varrho^2(q_1)]\sin\varpi(q_1)\right\} \, ,
\end{aligned} \tag{S154}$$

where we have defined

$$\varrho(q_1) \doteq (1-4q_1)\sqrt{-q_1}\,, \quad \varpi(q_1) \doteq \frac{2}{3}\varrho^3(q_1) - \frac{2}{3}(-q)^{3/2}\,. \tag{S155}$$

### C. Imperfect focusing in uniform medium

Let us consider a collimated beam propagating in vacuum along the $q_1$ direction. This situation is described by the two-dimensional paraxial equation [4]

$$i\partial_{q_1}\psi(q_1,q_2) + \frac{1}{2}\partial_{q_2}^2\psi(q_1,q_2) + \psi(q_1,q_2) = 0\,. \tag{S156}$$

Let us also consider the initial conditions

$$\psi(0,q_2) = \sqrt{\frac{2\pi i}{f}}\exp\left(-\frac{i}{2f}\,q_2^2 - \frac{ia}{4f^3}\,q_2^4\right)\,. \tag{S157}$$

This choice of initial conditions will produce a wave field that is focused at $(q_1,q_2) = (f,0)$, but with aberration determined by the parameter $a$. The case $a = 0$ corresponds to perfect focusing. When $a > 0$, the wave focuses prematurely, and the resultant cusp caustic points in the $+q_1$ direction. When $a < 0$, the wave focuses beyond the desired focal point, and the result cusp caustic points in the $-q_1$ direction. This is the case that we shall consider below, and we shall also assume $f \gg 1$. These conditions significantly simplify calculations.

#### 1. *Weyl symbol*

The wave equation can be equivalently written as

$$-\left(i\partial_{q_1} + \frac{1}{2}\partial_{q_2}^2 + 1\right)\int \mathrm{d}\mathbf{q}'\,\delta(\mathbf{q}-\mathbf{q}')\psi(\mathbf{q}') = \int \mathrm{d}\mathbf{q}'\,\left[-i\partial_{q_1}\delta(\mathbf{q}-\mathbf{q}') - \frac{1}{2}\partial_{q_2}^2\delta(\mathbf{q}-\mathbf{q}') - \delta(\mathbf{q}-\mathbf{q}')\right]\psi(\mathbf{q}')\,. \tag{S158}$$

Hence, the integration kernel is

$$D(\mathbf{q},\mathbf{q}') = -i\partial_{q_1-q_1'}\delta(\mathbf{q}-\mathbf{q}') - \frac{1}{2}\partial_{q_2-q_2'}^2\delta(\mathbf{q}-\mathbf{q}') - \delta(\mathbf{q}-\mathbf{q}')\,. \tag{S159}$$

We calculate the Weyl symbol as

$$\begin{aligned}\mathcal{D}(\mathbf{q},\mathbf{k}) \doteq \int \mathrm{d}\mathbf{s}\,e^{i\mathbf{k}^\intercal\mathbf{s}}\,D\left(\mathbf{q}-\frac{\mathbf{s}}{2},\mathbf{q}+\frac{\mathbf{s}}{2}\right) &= \int \mathrm{d}\mathbf{s}\,e^{i\mathbf{k}^\intercal\mathbf{s}}\,\left[-i\partial_{-s_1}\delta(-\mathbf{s}) - \frac{1}{2}\partial_{-s_2}^2\delta(-\mathbf{s}) - \delta(-\mathbf{s})\right]\\ &= \int \mathrm{d}\mathbf{s}\,e^{-i\mathbf{k}^\intercal\mathbf{s}}\,\left[-i\partial_{s_1}\delta(\mathbf{s}) - \frac{1}{2}\partial_{s_2}^2\delta(\mathbf{s}) - \delta(\mathbf{s})\right]\\ &= k_1 + \frac{k_2^2}{2} - 1\,.\end{aligned} \tag{S160}$$

#### 2. *Ray tracing*

The ray equations are

$$\partial_{\tau_1}k_1(\boldsymbol{\tau}) = -\partial_{q_1}\mathcal{D}\left[\mathbf{q}(\boldsymbol{\tau}),\mathbf{k}(\boldsymbol{\tau})\right] = 0\,, \quad \partial_{\tau_1}q_1(\boldsymbol{\tau}) = \partial_{k_1}\mathcal{D}\left[\mathbf{q}(\boldsymbol{\tau}),\mathbf{k}(\boldsymbol{\tau})\right] = 1\,, \tag{S161a}$$

$$\partial_{\tau_1}k_2(\boldsymbol{\tau}) = -\partial_{q_2}\mathcal{D}\left[\mathbf{q}(\boldsymbol{\tau}),\mathbf{k}(\boldsymbol{\tau})\right] = 0\,, \quad \partial_{\tau_1}q_2(\boldsymbol{\tau}) = \partial_{k_2}\mathcal{D}\left[\mathbf{q}(\boldsymbol{\tau}),\mathbf{k}(\boldsymbol{\tau})\right] = k_2(\boldsymbol{\tau})\,. \tag{S161b}$$

The solution is

$$k_1(\boldsymbol{\tau}) = k_1(0,\tau_2)\,, \quad q_1(\boldsymbol{\tau}) = q_1(0,\tau_2) + \tau_1\,, \tag{S162a}$$

$$k_2(\boldsymbol{\tau}) = k_2(0,\tau_2)\,, \quad q_2(\boldsymbol{\tau}) = q_2(0,\tau_2) + k_2(0,\tau_2)\,\tau_1\,. \tag{S162b}$$

Since our initial condition for $\psi$ are specified on the surface $q_1 = 0$, it is natural to choose $q_1(0, \tau_2) = 0$. The functions $k_1(0, \tau_2)$ and $k_2(0, \tau_2)$ are then determined respectively by the local dispersion relation and the initial condition for $\psi$, and only $q_2(0, \tau_2)$ remains undetermined. Since $\tau_2$ parameterizes the initial ray conditions, let us choose $q_2(0, \tau_2) = f\tau_2$. Then, the above solutions can be written as

$$k_1(\boldsymbol{\tau}) = k_1(0, \tau_2) \, , \quad q_1(\boldsymbol{\tau}) = \tau_1 \, , \tag{S163a}$$

$$k_2(\boldsymbol{\tau}) = k_2(0, \tau_2) \, , \quad q_2(\boldsymbol{\tau}) = f\tau_2 + k_2(0, \tau_2)\, \tau_1 \, . \tag{S163b}$$

We compute the initial wavevector $k_2(0, \tau_2)$ using the initial field conditions

$$k_2(0, \tau_2) = \partial_{q_2} \left( -\frac{1}{2f}\, q_2^2 - \frac{a}{4f^3}\, q_2^4 \right)\bigg|_{q_2(0,\tau_2)} = -\frac{q_2}{f} - a\frac{q_2^3}{f^3}\bigg|_{q_2(0,\tau_2)} = -\tau_2 - a\, \tau_2^3 \, . \tag{S164}$$

Then, the initial $k_1(0, \tau_2)$ is determined from $\mathcal{D}[\mathbf{q}(0, \tau_2), \mathbf{k}(0, \tau_2)] = 0$ to be

$$k_1(0, \tau_2) = 1 - \frac{k_2^2(0, \tau_2)}{2} \, . \tag{S165}$$

Therefore we obtain the ray solutions

$$q_1(\boldsymbol{\tau}) = \tau_1 \, , \tag{S166a}$$

$$q_2(\boldsymbol{\tau}) = f\tau_2 + k_2(\tau_2)\tau_1 \, , \tag{S166b}$$

$$k_1(\boldsymbol{\tau}) = 1 - \frac{[k_2(\tau_2)]^2}{2} \, , \tag{S166c}$$

$$k_2(\tau_2) = -\,\tau_2 - a\, \tau_2^3 \, . \tag{S166d}$$

Note also that

$$j_{\boldsymbol{\tau}} = \det \partial_{\boldsymbol{\tau}} \mathbf{q} = f + \tau_1 k_2'(\tau_2) \, . \tag{S167}$$

We next construct $\boldsymbol{\tau}(\mathbf{q})$. Clearly,

$$\tau_1(\mathbf{q}) = q_1 \, . \tag{S168}$$

Hence, we must solve

$$a q_1 \tau_2^3 + (q_1 - f)\tau_2 + q_2 = 0 \, . \tag{S169}$$

Let us define the discriminant as

$$\Delta(\mathbf{q}) \doteq 4 \left( \frac{q_1 - f}{a q_1} \right)^3 + 27 \left( \frac{q_2}{a q_1} \right)^2 \, . \tag{S170}$$

Then, where $\Delta(\mathbf{q}) > 0$, there is only one real root, given by

$$\tau_2^{(0)}(\mathbf{q}) = \left( -\frac{q_2}{2 a q_1} + \sqrt{\frac{\Delta(\mathbf{q})}{108}} \right)^{1/3} + \left( -\frac{q_2}{2 a q_1} - \sqrt{\frac{\Delta(\mathbf{q})}{108}} \right)^{1/3} \, , \tag{S171}$$

and where $\Delta(\mathbf{q}) \leq 0$, there are two additional real roots, given by

$$\tau_2^{(\pm)}(\mathbf{q}) = \mathrm{Re} \left[ (-1 \pm i\sqrt{3}) \left( -\frac{q_2}{2 a q_1} + i \sqrt{\frac{|\Delta(\mathbf{q})|}{108}} \right)^{1/3} \right] \, . \tag{S172}$$

### *3. Tangent-space transformation matrix*

We now perform symplectic Gram–Schmidt algorithm to obtain $\mathsf{S}_{\mathbf{t}}$. First, let us define

$$\vartheta_{\mathbf{t}} \doteq \sqrt{1 + k_2^2(t_2)} \, , \quad \varphi_{\mathbf{t}} \doteq \sqrt{j_{\mathbf{t}}^2 + [k_2'(t_2)\vartheta_{\mathbf{t}}^2]^2} \, . \tag{S173}$$

Then, upon calculating the derivatives

$$\partial_{t_1}\mathbf{z}(\mathbf{t}) = \begin{pmatrix} 1 \\ k_2(t_2) \\ 0 \\ 0 \end{pmatrix} \, , \quad \partial_{t_2}\mathbf{z}(\mathbf{t}) = \begin{pmatrix} 0 \\ j_{\mathbf{t}} \\ -k_2(t_2)k_2'(t_2) \\ k_2'(t_2) \end{pmatrix} \, , \tag{S174}$$

we compute

$$\check{\mathbf{T}}_1(\mathbf{t}) = \frac{\partial_{\tau_1}\mathbf{z}(\mathbf{t})}{\|\partial_{\tau_1}\mathbf{z}(\mathbf{t})\|} = \frac{1}{\vartheta_{\mathbf{t}}} \begin{pmatrix} 1 \\ k_2(t_2) \\ 0 \\ 0 \end{pmatrix} \, , \tag{S175}$$

$$\check{\mathbf{T}}_2(\mathbf{t}) = \frac{\partial_{t_2}\mathbf{z}(\mathbf{t}) - [\check{\mathbf{T}}_1(\mathbf{t}) \cdot \partial_{t_2}\mathbf{z}(\mathbf{t})] \, \check{\mathbf{T}}_1(\mathbf{t})}{\|\partial_{t_2}\mathbf{z}(\mathbf{t}) - [\check{\mathbf{T}}_1(\mathbf{t}) \cdot \partial_{t_2}\mathbf{z}(\mathbf{t})] \, \check{\mathbf{T}}_1(\mathbf{t})\|} = \frac{1}{\vartheta_{\mathbf{t}}\varphi_{\mathbf{t}}} \begin{pmatrix} -k_2(t_2)j_{\mathbf{t}} \\ j_{\mathbf{t}} \\ -\vartheta_{\mathbf{t}}^2 k_2(t_2)\, k_2'(t_2) \\ \vartheta_{\mathbf{t}}^2\, k_2'(t_2) \end{pmatrix} . \tag{S176}$$

Hence, we compute the normal vectors

$$\check{\mathbf{N}}_1(\mathbf{t}) = -\mathsf{J}\check{\mathbf{T}}_1(\mathbf{t}) = \frac{1}{\vartheta_{\mathbf{t}}} \begin{pmatrix} 0 \\ 0 \\ 1 \\ k_2(t_2) \end{pmatrix} \, , \quad \check{\mathbf{N}}_2(\mathbf{t}) = -\mathsf{J}\check{\mathbf{T}}_2(\mathbf{t}) = \frac{1}{\vartheta_{\mathbf{t}}\varphi_{\mathbf{t}}} \begin{pmatrix} \vartheta_{\mathbf{t}}^2 k_2(t_2)\, k_2'(t_2) \\ -\vartheta_{\mathbf{t}}^2\, k_2'(t_2) \\ -k_2(t_2)j_{\mathbf{t}} \\ j_{\mathbf{t}} \end{pmatrix} . \tag{S177}$$

We therefore construct $\mathsf{S}_{\mathbf{t}}$ to be

$$\mathsf{S}_{\mathbf{t}} = \begin{pmatrix} \check{\mathbf{T}}_1^\intercal \\ \check{\mathbf{T}}_2^\intercal \\ \check{\mathbf{N}}_1^\intercal \\ \check{\mathbf{N}}_2^\intercal \end{pmatrix} = \frac{1}{\vartheta_{\mathbf{t}}\varphi_{\mathbf{t}}} \begin{pmatrix} \varphi_{\mathbf{t}} & k_2(t_2)\varphi_{\mathbf{t}} & 0 & 0 \\ -k_2(t_2)j_{\mathbf{t}} & j_{\mathbf{t}} & -\vartheta_{\mathbf{t}}^2 k_2(t_2)\, k_2'(t_2) & \vartheta_{\mathbf{t}}^2\, k_2'(t_2) \\ 0 & 0 & \varphi_{\mathbf{t}} & k_2(t_2)\varphi_{\mathbf{t}} \\ \vartheta_{\mathbf{t}}^2 k_2(t_2)\, k_2'(t_2) & -\vartheta_{\mathbf{t}}^2\, k_2'(t_2) & -k_2(t_2)j_{\mathbf{t}} & j_{\mathbf{t}} \end{pmatrix} , \tag{S178}$$

and we subsequently identify the submatrices

$$\mathsf{A}_{\mathbf{t}} = \mathsf{D}_{\mathbf{t}} = \frac{1}{\vartheta_{\mathbf{t}}\varphi_{\mathbf{t}}} \begin{pmatrix} \varphi_{\mathbf{t}} & k_2(t_2)\varphi_{\mathbf{t}} \\ -k_2(t_2)j_{\mathbf{t}} & j_{\mathbf{t}} \end{pmatrix} \, , \quad \mathsf{B}_{\mathbf{t}} = -\mathsf{C}_{\mathbf{t}} = \frac{\vartheta_{\mathbf{t}} k_2'(t_2)}{\varphi_{\mathbf{t}}} \begin{pmatrix} 0 & 0 \\ -k_2(t_2) & 1 \end{pmatrix} . \tag{S179}$$

### *4. Tangent-space rays*

The tangent-space rays are obtained as

$$\mathbf{Q}_{\mathbf{t}}(\boldsymbol{\tau}) = \mathsf{A}_{\mathbf{t}}\mathbf{q}(\boldsymbol{\tau}) + \mathsf{B}_{\mathbf{t}}\mathbf{k}(\boldsymbol{\tau}) \, , \quad \mathbf{K}_{\mathbf{t}}(\boldsymbol{\tau}) = \mathsf{C}_{\mathbf{t}}\mathbf{q}(\boldsymbol{\tau}) + \mathsf{D}_{\mathbf{t}}\mathbf{k}(\boldsymbol{\tau}) \, . \tag{S180}$$

Notably,

$$\mathbf{Q}_{\mathbf{t}}(\mathbf{t}) = \frac{1}{2\vartheta_{\mathbf{t}}\varphi_{\mathbf{t}}} \begin{pmatrix} 2\varphi_{\mathbf{t}}[f t_2 k_2(t_2) + t_1\vartheta_{\mathbf{t}}^2] \\ 2 f t_2 j_{\mathbf{t}} + \vartheta_{\mathbf{t}}^2 k_2^3(t_2) k_2'(t_2) \end{pmatrix} \, , \quad \mathbf{K}_{\mathbf{t}}(\mathbf{t}) = \frac{1}{2\vartheta_{\mathbf{t}}\varphi_{\mathbf{t}}} \begin{pmatrix} \varphi_{\mathbf{t}}[1 + \vartheta_{\mathbf{t}}^2] \\ k_2^3(t_2) j_{\mathbf{t}} - 2 f t_2 \vartheta_{\mathbf{t}}^2 k_2'(t_2) \end{pmatrix} \, , \tag{S181}$$

and

$$\partial_{t_1}\mathbf{Q}_{\mathbf{t}}(\mathbf{t}) = \frac{1}{2\varphi_{\mathbf{t}}^3} \begin{pmatrix} 2\varphi_{\mathbf{t}}^3\vartheta_{\mathbf{t}} \\ \vartheta_{\mathbf{t}}[k_2'(t_2)]^2[2 f t_2 \vartheta_{\mathbf{t}}^2 k_2'(t_2) - k_2^3(t_2) j_{\mathbf{t}}] \end{pmatrix} . \tag{S182}$$

### 5. *Tangent-space envelope*

We first compute

$$\partial_{\boldsymbol{\tau}} \mathbf{Q}_{\mathbf{t}}(\boldsymbol{\tau}) = \begin{pmatrix} \partial_{\tau_1} Q_{\mathbf{t},1}(\boldsymbol{\tau}) & \partial_{\tau_1} Q_{\mathbf{t},2}(\boldsymbol{\tau}) \\ \partial_{\tau_2} Q_{\mathbf{t},1}(\boldsymbol{\tau}) & \partial_{\tau_2} Q_{\mathbf{t},2}(\boldsymbol{\tau}) \end{pmatrix}$$
$$= \frac{1}{\vartheta_{\mathbf{t}} \varphi_{\mathbf{t}}} \begin{pmatrix} \varphi_{\mathbf{t}}[1 + k_2(t_2) k_2(\tau_2)] & j_{\mathbf{t}}[k_2(\tau_2) - k_2(t_2)] \\ \varphi_{\mathbf{t}} j_{\boldsymbol{\tau}} k_2(t_2) & j_{\mathbf{t}} j_{\boldsymbol{\tau}} + \vartheta_{\mathbf{t}}^2 k_2'(t_2) k_2'(\tau_2)[1 + k_2(t_2) k_2(\tau_2)] \end{pmatrix} . \tag{S183}$$

Hence, we compute

$$J_{\mathbf{t}}(\boldsymbol{\tau}) = \det \partial_{\boldsymbol{\tau}} \mathbf{Q}_{\mathbf{t}}(\boldsymbol{\tau}) = \frac{j_{\mathbf{t}} j_{\boldsymbol{\tau}} + [1 + k_2(t_2) k_2(\tau_2)]^2 k_2'(\tau_2) k_2'(t_2)}{\varphi_{\mathbf{t}}} . \tag{S184}$$

Since $J_{\mathbf{t}}(\boldsymbol{\tau}) = \varphi_{\mathbf{t}}$, we obtain

$$\Phi_{\mathbf{t}}[\mathbf{Q}_{\mathbf{t}}(\boldsymbol{\tau})] = \Phi_{\mathbf{t}}[\mathbf{Q}_{\mathbf{t}}(t_1, \tau_2)] \frac{\varphi_{\mathbf{t}}}{\sqrt{j_{\mathbf{t}} j_{\boldsymbol{\tau}} + [1 + k_2(t_2) k_2(\tau_2)]^2 k_2'(\tau_2) k_2'(t_2)}} . \tag{S185}$$

For simplicity, let us choose $\Phi_{\mathbf{t}}[\mathbf{Q}_{\mathbf{t}}(t_1, \tau_2)] = 1$. Then,

$$\Phi_{\mathbf{t}}[\mathbf{Q}_{\mathbf{t}}(\boldsymbol{\tau})] = \frac{\varphi_{\mathbf{t}}}{\sqrt{j_{\mathbf{t}} j_{\boldsymbol{\tau}} + [1 + k_2(t_2) k_2(\tau_2)]^2 k_2'(\tau_2) k_2'(t_2)}} . \tag{S186}$$

We calculate

$$\partial_{\boldsymbol{\tau}} \Phi_{\mathbf{t}}[\mathbf{Q}_{\mathbf{t}}(\mathbf{t})] = \left. \begin{pmatrix} \partial_{\tau_1} \Phi_{\mathbf{t}}[\mathbf{Q}_{\mathbf{t}}(\boldsymbol{\tau})] \\ \partial_{\tau_2} \Phi_{\mathbf{t}}[\mathbf{Q}_{\mathbf{t}}(\boldsymbol{\tau})] \end{pmatrix} \right|_{\boldsymbol{\tau} = \mathbf{t}}$$
$$= -\frac{1}{2\varphi_{\mathbf{t}}^2} \begin{pmatrix} j_{\mathbf{t}} k_2'(t_2) \\ 2\vartheta_{\mathbf{t}}^2 k_2(t_2)[k_2'(t_2)]^3 + [t_1 j_{\mathbf{t}} + \vartheta_{\mathbf{t}}^4 k_2'(t_2)] k_2''(t_2) \end{pmatrix} . \tag{S187}$$

Upon invoking the inverse function theorem, we compute

$$\partial_{\mathbf{Q}} \Phi_{\mathbf{t}}[\mathbf{Q}_{\mathbf{t}}(\mathbf{t})] = \begin{pmatrix} \partial_{Q_{\mathbf{t},1}} \tau_1(\mathbf{Q}_{\mathbf{t}}) & \partial_{Q_{\mathbf{t},1}} \tau_2(\mathbf{Q}_{\mathbf{t}}) \\ \partial_{Q_{\mathbf{t},2}} \tau_1(\mathbf{Q}_{\mathbf{t}}) & \partial_{Q_{\mathbf{t},2}} \tau_2(\mathbf{Q}_{\mathbf{t}}) \end{pmatrix} \begin{pmatrix} \partial_{\tau_1} \Phi_{\mathbf{t}}[\mathbf{Q}_{\mathbf{t}}(\mathbf{t})] \\ \partial_{\tau_1} \Phi_{\mathbf{t}}[\mathbf{Q}_{\mathbf{t}}(\mathbf{t})] \end{pmatrix}$$
$$= \begin{pmatrix} \partial_{\tau_1} Q_{\mathbf{t},1}(\mathbf{t}) & \partial_{\tau_1} Q_{\mathbf{t},2}(\mathbf{t}) \\ \partial_{\tau_2} Q_{\mathbf{t},1}(\mathbf{t}) & \partial_{\tau_2} Q_{\mathbf{t},2}(\mathbf{t}) \end{pmatrix}^{-1} \begin{pmatrix} \partial_{\tau_1} \Phi_{\mathbf{t}}[\mathbf{Q}_{\mathbf{t}}(\mathbf{t})] \\ \partial_{\tau_1} \Phi_{\mathbf{t}}[\mathbf{Q}_{\mathbf{t}}(\mathbf{t})] \end{pmatrix}$$
$$= \frac{1}{2\vartheta_{\mathbf{t}} \varphi_{\mathbf{t}}^3} \begin{pmatrix} -j_{\mathbf{t}} \varphi_{\mathbf{t}} k_2'(t_2) \\ (3j_{\mathbf{t}}^2 - 2\varphi_{\mathbf{t}}^2) k_2(t_2) k_2'(t_2) - [t_1 j_{\mathbf{t}} + \vartheta_{\mathbf{t}}^4 k_2'(t_2)] \vartheta_{\mathbf{t}}^2 k_2''(t_2) \end{pmatrix} . \tag{S188}$$

### 6. *Linking with NIMT*

We compute

$$(\partial_{t_1} \mathsf{S}_{\mathbf{t}}) \, \mathsf{S}_{\mathbf{t}}^{-1} = \frac{1}{\varphi_{\mathbf{t}}^2} \begin{pmatrix} 0 & 0 & 0 & 0 \\ 0 & 0 & 0 & -[k_2'(t_2)]^2 \vartheta_{\mathbf{t}}^2 \\ 0 & 0 & 0 & 0 \\ 0 & [k_2'(t_2)]^2 \vartheta_{\mathbf{t}}^2 & 0 & 0 \end{pmatrix} . \tag{S189}$$

Hence, we identify

$$\mathsf{V}_{\mathbf{t}} = \mathsf{0}_2 \, , \quad \mathsf{U}_{\mathbf{t}} = \mathsf{W}_{\mathbf{t}} = \frac{1}{\varphi_{\mathbf{t}}^2} \begin{pmatrix} 0 & 0 \\ 0 & -[k_2'(t_2)]^2 \vartheta_{\mathbf{t}}^2 \end{pmatrix} . \tag{S190}$$

We therefore obtain the simplification

$$\eta_{\mathbf{t}} \doteq \frac{i}{2} \left[ \mathbf{K}_{\mathbf{t}}^{\intercal}(\mathbf{t}) \mathsf{W}_{\mathbf{t}} \mathbf{K}_{\mathbf{t}}(\mathbf{t}) - \mathbf{Q}_{\mathbf{t}}^{\intercal}(\mathbf{t}) \mathsf{U}_{\mathbf{t}} \mathbf{Q}_{\mathbf{t}}(\mathbf{t}) + i \, \mathrm{tr}\,(\mathsf{V}_{\mathbf{t}}) \right] + \left[ \partial_h \mathbf{Q}_{\mathbf{t}}(\mathbf{t}) - \mathsf{V}_{\mathbf{t}}^{\intercal} \mathbf{Q}_{\mathbf{t}}(\mathbf{t}) - \mathsf{W}_{\mathbf{t}}^{\intercal} \mathbf{K}_{\mathbf{t}}(\mathbf{t}) \right]^{\intercal} \left\{ \partial_{\mathbf{Q}} \Phi_{\mathbf{t}} \left[ \mathbf{Q}_{\mathbf{t}}(\mathbf{t}) \right] + i \mathbf{K}_{\mathbf{t}}(\mathbf{t}) \right\}$$
$$= \frac{i}{2} \left[ \mathbf{K}_{\mathbf{t}}^{\intercal}(\mathbf{t}) \mathsf{W}_{\mathbf{t}} \mathbf{K}_{\mathbf{t}}(\mathbf{t}) - \mathbf{Q}_{\mathbf{t}}^{\intercal}(\mathbf{t}) \mathsf{U}_{\mathbf{t}} \mathbf{Q}_{\mathbf{t}}(\mathbf{t}) \right] + \left[ \partial_h \mathbf{Q}_{\mathbf{t}}(\mathbf{t}) - \mathsf{W}_{\mathbf{t}}^{\intercal} \mathbf{K}_{\mathbf{t}}(\mathbf{t}) \right]^{\intercal} \left\{ \partial_{\mathbf{Q}} \Phi_{\mathbf{t}} \left[ \mathbf{Q}_{\mathbf{t}}(\mathbf{t}) \right] + i \mathbf{K}_{\mathbf{t}}(\mathbf{t}) \right\}$$
$$= -\frac{j_{\mathbf{t}} k_2'(t_2)}{2\varphi_{\mathbf{t}}^2} + i \frac{1 + \vartheta_{\mathbf{t}}^2}{2} + i \frac{[4f^2 t_2^2 - k_2^6(t_2)](2j_{\mathbf{t}}^2 - \varphi_{\mathbf{t}}^2)[k_2'(t_2)]^2}{8\varphi_{\mathbf{t}}^4} + i \frac{f t_2 \vartheta_{\mathbf{t}}^2 j_{\mathbf{t}} k_2^3(t_2)[k_2'(t_2)]^3}{\varphi_{\mathbf{t}}^4} . \tag{S191}$$

Integrating $\eta_{\mathbf{t}}$ along the rays yields

$$-\int_0^{t_1} \mathrm{d}h \, \frac{[f + hk_2'(t_2)]k_2'(t_2)}{2\vartheta_{\mathbf{t}}^4[k_2'(t_2)]^2 + 2[f + hk_2'(t_2)]^2} = \log \sqrt{\frac{\varphi_{(0,t_2)}}{\varphi_{\mathbf{t}}}} \,, \tag{S192a}$$

$$i\int_0^{t_1} \mathrm{d}h \, \frac{1 + \vartheta_{\mathbf{t}}^2}{2} = it_1 \frac{1 + \vartheta_{\mathbf{t}}^2}{2} \,, \tag{S192b}$$

$$i\int_0^{t_1} \mathrm{d}h \, \frac{[4f^2t_2^2 - k_2^6(t_2)](2j_{\mathbf{t}}^2 - \varphi_{\mathbf{t}}^2)[k_2'(t_2)]^2}{8\varphi_{\mathbf{t}}^4} = i[k_2'(t_2)]^2 \frac{4f^2t_2^2 - k_2^6(t_2)}{8} \frac{[2f^2 - \varphi_{(0,t_2)}^2]t_1 + fk_2'(t_2)t_1^2}{\varphi_{\mathbf{t}}^2\varphi_{(0,t_2)}^2} \,, \tag{S192c}$$

$$i\int_0^{t_1} \mathrm{d}h \, \frac{ft_2\vartheta_{\mathbf{t}}^2 j_{\mathbf{t}} k_2^3(t_2)[k_2'(t_2)]^3}{\varphi_{\mathbf{t}}^4} = ift_1t_2\vartheta_{\mathbf{t}}^2[k_2(t_2)k_2'(t_2)]^3 \frac{f + j_{\mathbf{t}}}{2\varphi_{\mathbf{t}}^2\varphi_{(0,t_2)}^2} \,. \tag{S192d}$$

Therefore, we obtain

$$\begin{aligned} \alpha_{\mathbf{t}} &= \alpha_{(0,t_2)}\sqrt{\frac{\varphi_{(0,t_2)}}{\varphi_{\mathbf{t}}}} \exp\left(i\chi_{\mathbf{t}}\right) \,, \\ \chi_{\mathbf{t}} &= t_1\frac{1+\vartheta_{\mathbf{t}}^2}{2} + [k_2'(t_2)]^2 \frac{4f^2t_2^2 - k_2^6(t_2)}{8} \frac{[2f^2 - \varphi_{(0,t_2)}^2]t_1 + fk_2'(t_2)t_1^2}{\varphi_{\mathbf{t}}^2\varphi_{(0,t_2)}^2} + ft_1t_2\vartheta_{\mathbf{t}}^2[k_2(t_2)k_2'(t_2)]^3 \frac{f + j_{\mathbf{t}}}{2\varphi_{\mathbf{t}}^2\varphi_{(0,t_2)}^2} \,, \end{aligned} \tag{S193}$$

where $\alpha_{(0,t_2)}$ is a function of $t_2$ determined by the initial conditions.

### 7. *Inverse MT*

It is difficult to directly compute $\Theta_{\mathbf{t}}(\mathbf{Q})$ via Eq. (29) of the main text, as was done in the previous examples. Instead, we shall first set up the inverse MT integral, then approximate $\Theta_{\mathbf{t}}(\mathbf{Q})$ in the desired limit. Therefore, we perform the SVD of $\mathsf{B}$ to obtain

$$\mathsf{B}_{\mathbf{t}} = \begin{pmatrix} 0 & 1 \\ -1 & 0 \end{pmatrix} \begin{pmatrix} \frac{\vartheta_{\mathbf{t}}^2 k_2'(t_2)}{\varphi_{\mathbf{t}}} & 0 \\ 0 & 0 \end{pmatrix} \begin{pmatrix} \frac{k_2(t_2)}{\vartheta_{\mathbf{t}}} & -\frac{1}{\vartheta_{\mathbf{t}}} \\ \frac{1}{\vartheta_{\mathbf{t}}} & \frac{k_2(t_2)}{\vartheta_{\mathbf{t}}} \end{pmatrix} \,. \tag{S194}$$

Hence, we identify

$$\mathsf{L} = \begin{pmatrix} 0 & 1 \\ -1 & 0 \end{pmatrix} \,, \quad \mathsf{R} = \frac{1}{\vartheta_{\mathbf{t}}} \begin{pmatrix} k_2(t_2) & 1 \\ -1 & k_2(t_2) \end{pmatrix} \,, \tag{S195}$$

and one can verify that $\det \mathsf{L} = \det \mathsf{R} = 1$. Correspondingly, we obtain

$$\widetilde{\mathsf{A}} = \widetilde{\mathsf{D}} = \frac{1}{\varphi_{\mathbf{t}}} \begin{pmatrix} j_{\mathbf{t}} & 0 \\ 0 & \varphi_{\mathbf{t}} \end{pmatrix} \,, \quad \widetilde{\mathsf{B}} = -\widetilde{\mathsf{C}} = \frac{1}{\varphi_{\mathbf{t}}} \begin{pmatrix} \vartheta_{\mathbf{t}}^2 k_2'(t_2) & 0 \\ 0 & 0 \end{pmatrix} \,. \tag{S196}$$

Clearly, $\rho = 1$. Hence, we obtain

$$\psi_{\mathbf{t}}(\mathbf{q}) = \frac{\sigma_{\mathbf{t}}\, \alpha_{\mathbf{t}} \exp\left[-\frac{i}{2}\beta_{\mathbf{t}}^\rho(\mathbf{q})\right]}{(-2\pi i)^{\rho/2}\sqrt{\det \Lambda_{\rho\rho} \det \mathsf{a}_{\varsigma\varsigma}^{-1}}} \Upsilon_{\mathbf{t}}^\rho(\mathbf{q}) = \frac{\sigma_{\mathbf{t}}\, \alpha_{\mathbf{t}} \exp\left[-\frac{i}{2}\beta_{\mathbf{t}}^\rho(\mathbf{q})\right]}{\sqrt{-2\pi i}\sqrt{\frac{\vartheta_{\mathbf{t}}^2 k_2'(t_2)}{\varphi_{\mathbf{t}}}}} \Upsilon_{\mathbf{t}}^\rho(\mathbf{q}) \,, \tag{S197}$$

or, plugging in our result for $\alpha_{\mathbf{t}}$,

$$\psi_{\mathbf{t}}(\mathbf{q}) = \frac{\sigma_{\mathbf{t}}\, \alpha_{(0,t_2)}\sqrt{\varphi_{(0,t_2)}}}{\vartheta_{\mathbf{t}}\sqrt{-2\pi i}\sqrt{k_2'(t_2)}} \exp\left[i\chi_{\mathbf{t}} - \frac{i}{2}\beta_{\mathbf{t}}^\rho(\mathbf{q})\right] \Upsilon_{\mathbf{t}}^\rho(\mathbf{q}) \,. \tag{S198}$$

Note that $k_2'(t_2)$ can change sign, which means that the branch cut of the MT can be crossed. Hence, $\sigma_{\mathbf{t}} = \sigma_{t_2} \neq 1$. However, we do not need to explicitly compute $\sigma_{t_2}$, since it will be removed by matching to initial conditions.

We next calculate

$$\mathsf{M}_3 = \begin{pmatrix} \frac{\varphi_{\mathbf{t}}}{\vartheta_{\mathbf{t}}^2 k_2'(t_2)} & 0 \end{pmatrix} \,, \quad \mathsf{M}_4 = \begin{pmatrix} \frac{j_{\mathbf{t}}}{\vartheta_{\mathbf{t}}^2 k_2'(t_2)} & 0 \\ 0 & 0 \end{pmatrix} \,. \tag{S199}$$

Then, since

$$\check{\boldsymbol{\ell}}_\rho = \begin{pmatrix} 0 & -1 \end{pmatrix} , \quad \check{\boldsymbol{\ell}}_{\rho+1} = \begin{pmatrix} 1 & 0 \end{pmatrix} , \quad \check{\mathbf{r}}_\rho = \begin{pmatrix} \frac{k_2(t_2)}{\vartheta_{\mathbf{t}}} & -\frac{1}{\vartheta_{\mathbf{t}}} \end{pmatrix} , \quad \check{\mathbf{r}}_{\rho+1} = \begin{pmatrix} \frac{1}{\vartheta_{\mathbf{t}}} & \frac{k_2(t_2)}{\vartheta_{\mathbf{t}}} \end{pmatrix} , \tag{S200}$$

we obtain

$$\mathbf{Q}_\rho = -Q_{\mathbf{t},2} , \quad \mathbf{Q}_\varsigma = Q_{\mathbf{t},1} . \tag{S201}$$

Therefore,

$$\begin{aligned} \beta^\rho_{\mathbf{t}}[\mathbf{q}(\mathbf{t})] &\doteq \mathbf{q}^\intercal(\mathbf{t}) \, \mathsf{R}\mathsf{M}_4\mathsf{R}^\intercal \mathbf{q}(\mathbf{t}) - 2 \left[\mathbf{Q}^\rho_{\mathbf{t}}(\mathbf{t})\right]^\intercal \, \mathsf{M}_3\mathsf{R}^\intercal\mathbf{q}(\mathbf{t}) + \left[\mathbf{Q}^\rho_{\mathbf{t}}(\mathbf{t})\right]^\intercal \, \mathsf{d}_{\rho\rho}\mathsf{\Lambda}^{-1}_{\rho\rho} \, \mathbf{Q}^\rho_{\mathbf{t}}(\mathbf{t}) \\ &= \frac{f^2 j_{\mathbf{t}} t_2^2 - 2f\varphi_{\mathbf{t}}\vartheta_{\mathbf{t}} t_2 \, Q_{\mathbf{t},2}(\mathbf{t}) + j_{\mathbf{t}}\vartheta^2_{\mathbf{t}} \, Q^2_{\mathbf{t},2}(\mathbf{t})}{\vartheta^4_{\mathbf{t}} k'_2(t_2)} , \end{aligned} \tag{S202}$$

$$\begin{aligned} \gamma^\rho_{\mathbf{t}}[\epsilon_\rho, \mathbf{q}(\mathbf{t})] &\doteq \frac{1}{2}\boldsymbol{\epsilon}^\intercal_\rho \, \mathsf{d}_{\rho\rho}\mathsf{\Lambda}^{-1}_{\rho\rho} \, \boldsymbol{\epsilon}_\rho + \boldsymbol{\epsilon}^\intercal_\rho \left[\mathsf{d}_{\rho\rho}\mathsf{\Lambda}^{-1}_{\rho\rho}\mathbf{Q}^\rho_{\mathbf{t}}(\mathbf{t}) - \mathsf{M}_3\mathsf{R}^\intercal\mathbf{q}\right] \\ &= \frac{j_{\mathbf{t}}}{2\vartheta^2_{\mathbf{t}} k'_2(t_2)}\epsilon^2_\rho - K_{\mathbf{t},2}(\mathbf{t})\epsilon_\rho . \end{aligned} \tag{S203}$$

We next calculate $\Upsilon^\rho_{\mathbf{t}}$. By definition,

$$\begin{aligned} \Upsilon^\rho_{\mathbf{t}}[\mathbf{q}(\mathbf{t})] &\doteq \int_{\mathcal{C}_0} \mathrm{d}\epsilon_\rho \, \Psi_{\mathbf{t}} \left[\mathsf{a}_{\varsigma\varsigma}\mathbf{q}_\varsigma(\mathbf{t}), Q_{\mathbf{t},2}(\mathbf{t}) - \epsilon_\rho\right] \exp\left\{-i\gamma^\rho_{\mathbf{t}}[\epsilon_\rho, \mathbf{q}(\mathbf{t})]\right\} \\ &= \int_{\mathcal{C}_0} \mathrm{d}\epsilon_\rho \, \Psi_{\mathbf{t}} \left[Q_{\mathbf{t},1}(\mathbf{t}), Q_{\mathbf{t},2}(\mathbf{t}) - \epsilon_\rho\right] \exp\left\{-i\gamma^\rho_{\mathbf{t}}[\epsilon_\rho, \mathbf{q}(\mathbf{t})]\right\} , \end{aligned} \tag{S204}$$

where we have used $\mathsf{a}_{\varsigma\varsigma}\mathbf{q}_\varsigma(\mathbf{t}) = Q_{\mathbf{t},1}(\mathbf{t})$. Let us approximate

$$\Phi_{\mathbf{t}} \left[Q_{\mathbf{t},1}(\mathbf{t}), Q_{\mathbf{t},2}(\mathbf{t}) - \epsilon_\rho\right] \approx \Phi_{\mathbf{t}} \left[Q_{\mathbf{t},1}(\mathbf{t}), Q_{\mathbf{t},2}(\mathbf{t})\right] = 1 . \tag{S205}$$

Then, the integral becomes

$$\begin{aligned} \Upsilon^\rho_{\mathbf{t}}[\mathbf{q}(\mathbf{t})] &\approx \int_{\mathcal{C}_0} \mathrm{d}\epsilon_\rho \, \exp\left\{i\Theta_{\mathbf{t}} \left[Q_{\mathbf{t},1}(\mathbf{t}), Q_{\mathbf{t},2}(\mathbf{t}) - \epsilon_\rho\right] - i\gamma^\rho_{\mathbf{t}}[\epsilon_\rho, \mathbf{q}(\mathbf{t})]\right\} \\ &\approx \int_{\mathcal{C}_0} \mathrm{d}\epsilon_\rho \, \exp\left\{-iK_{\mathbf{t},2}(\mathbf{t})\epsilon_\rho + \frac{i}{2}\partial_{Q_{\mathbf{t},2}}K_{\mathbf{t},2}(\mathbf{t})\epsilon^2_\rho - \frac{i}{6}\partial^2_{Q_{\mathbf{t},2}}K_{\mathbf{t},2}(\mathbf{t})\epsilon^3_\rho + \frac{i}{24}\partial^3_{Q_{\mathbf{t},2}}K_{\mathbf{t},2}(\mathbf{t})\epsilon^4_\rho - i\gamma^\rho_{\mathbf{t}}[\epsilon_\rho, \mathbf{q}(\mathbf{t})]\right\} \\ &= \int_{\mathcal{C}_0} \mathrm{d}\epsilon_\rho \, \exp\left\{i\left[\frac{1}{2}\partial_{Q_{\mathbf{t},2}}K_{\mathbf{t},2}(\mathbf{t}) - \frac{j_{\mathbf{t}}}{2\vartheta^2_{\mathbf{t}}k'_2(t_2)}\right]\epsilon^2_\rho - \frac{i}{6}\partial^2_{Q_{\mathbf{t},2}}K_{\mathbf{t},2}(\mathbf{t})\epsilon^3_\rho + \frac{i}{24}\partial^3_{Q_{\mathbf{t},2}}K_{\mathbf{t},2}(\mathbf{t})\epsilon^4_\rho\right\} . \end{aligned} \tag{S206}$$

### 8. *Taylor expansion of the tangent-space phase*

We must therefore calculate the derivatives of $K_{\mathbf{t},2}$ with respect to $Q_{\mathbf{t},2}$ at fixed $Q_{\mathbf{t},1} = Q_{\mathbf{t},1}(\mathbf{t})$. If we can find the constraint that $Q_{\mathbf{t},1}(\tau_1, \tau_2) = Q_{\mathbf{t},1}(\mathbf{t})$ imposes on $\tau_1$ and $\tau_2$, then we can perform the desired derivatives of $K_{\mathbf{t},2}$ implicitly along the constraint surface $\tau_{\mathbf{t},1}(\tau_2)$ or $\tau_{\mathbf{t},2}(\tau_1)$. Since

$$Q_{\mathbf{t},1}(\tau_1, \tau_2) = \frac{\tau_1[1 + k_2(t_2)k_2(\tau_2)] + f\tau_2 k_2(t_2)}{\vartheta_{\mathbf{t}}} , \tag{S207}$$

one can invert the relation $Q_{\mathbf{t},1}(\tau_1, \tau_2) = Q_{\mathbf{t},1}(\mathbf{t})$ to yield the constraint

$$\tau_{\mathbf{t},1}(\tau_2) = \frac{t_1\vartheta^2_{\mathbf{t}} + f(t_2 - \tau_2)k_2(t_2)}{1 + k_2(t_2)k_2(\tau_2)} . \tag{S208}$$

Hence, the functions $Q_{\mathbf{t},2}[\tau_{\mathbf{t},1}(\tau_2), \tau_2]$ and $K_{\mathbf{t},2}[\tau_{\mathbf{t},1}(\tau_2), \tau_2]$ both lie along the surface $Q_1 = Q_{\mathbf{t},1}(\mathbf{t})$. Since both $Q_{\mathbf{t},2}$ and $K_{\mathbf{t},2}$ can be considered univariate functions, i.e.,

$$K_{\mathbf{t},2}(\tau_2) \doteq K_{\mathbf{t},2}[\tau_{\mathbf{t},1}(\tau_2), \tau_2] , \quad Q_{\mathbf{t},2}(\tau_2) \doteq Q_{\mathbf{t},2}[\tau_{\mathbf{t},1}(\tau_2), \tau_2] , \tag{S209}$$

taking implicit derivatives is straightforward.

Indeed, taking $\partial_{Q_2}$ and $\partial^2_{Q_2}$ of the definition

$$Q_{\mathbf{t},2} = Q_{\mathbf{t},2}[\tau_{\mathbf{t},1}(\tau_2), \tau_2] \tag{S210}$$

yield the inversion relations between derivatives of $\tau_2$ and $Q_2$ at fixed $Q_1 = Q_{\mathbf{t},1}(\mathbf{t})$:

$$1 = \mathrm{d}_{\tau_2} Q_{\mathbf{t},2}\, \partial_{Q_2}\tau_2 \quad \to \quad \partial_{Q_2}\tau_2 = \frac{1}{\mathrm{d}_{\tau_2} Q_{\mathbf{t},2}}\,, \tag{S211a}$$

$$0 = \mathrm{d}^2_{\tau_2} Q_{\mathbf{t},2} (\partial_{Q_2}\tau_2)^2 + \mathrm{d}_{\tau_2} Q_{\mathbf{t},2} \partial^2_{Q_2}\tau_2 \quad \to \quad \partial^2_{Q_2}\tau_2 = -\frac{\mathrm{d}^2_{\tau_2} Q_{\mathbf{t},2}}{(\mathrm{d}_{\tau_2} Q_{\mathbf{t},2})^3}\,, \tag{S211b}$$

where $\mathrm{d}_{\tau_2} \doteq \partial_{\tau_2} + \partial_{\tau_2}\tau_{\mathbf{t},1}(\tau_2)\partial_{\tau_1}$ is the 'total' derivative with respect to $\tau_2$. Note also that

$$\mathrm{d}_{\tau_2} K_{\mathbf{t},2}(\mathbf{t}) = 0 \tag{S212}$$

by definition of the tangent plane. Hence, using Eqs. (S211) and (S212) we formally compute the first derivative

$$\partial_{Q_{\mathbf{t},2}} K_{\mathbf{t},2}(\mathbf{t}) = \frac{\mathrm{d}_{\tau_2} K_{\mathbf{t},2}(\mathbf{t})}{\mathrm{d}_{\tau_2} Q_{\mathbf{t},2}(\mathbf{t})} = 0\,, \tag{S213a}$$

the second derivative

$$\begin{aligned}
\partial^2_{Q_{\mathbf{t},2}} K_{\mathbf{t},2}(\mathbf{t}) &= \mathrm{d}^2_{\tau_2} K_{\mathbf{t},2}(\mathbf{t}) \{\partial_{Q_2}\tau_2[Q_{\mathbf{t},2}(\mathbf{t})]\}^2 + \mathrm{d}_{\tau_2} K_{\mathbf{t},2}(\mathbf{t})\, \partial^2_{Q_2}\tau_2[Q_{\mathbf{t},2}(\mathbf{t})] \\
&= \mathrm{d}^2_{\tau_2} K_{\mathbf{t},2}(\mathbf{t}) \{\partial_{Q_2}\tau_2[Q_{\mathbf{t},2}(\mathbf{t})]\}^2 \\
&= \frac{\mathrm{d}^2_{\tau_2} K_{\mathbf{t},2}(\mathbf{t})}{[\mathrm{d}_{\tau_2} Q_{\mathbf{t},2}(\mathbf{t})]^2}\,,
\end{aligned} \tag{S213b}$$

and the third derivative

$$\begin{aligned}
\partial^3_{Q_{\mathbf{t},2}} K_{\mathbf{t},2}(\mathbf{t}) &= \mathrm{d}^3_{\tau_2} K_{\mathbf{t},2}(\mathbf{t}) \{\partial_{Q_2}\tau_2[Q_{\mathbf{t},2}(\mathbf{t})]\}^3 + 3\, \mathrm{d}^2_{\tau_2} K_{\mathbf{t},2}(\mathbf{t})\, \partial^2_{Q_2}\tau_2[Q_{\mathbf{t},2}(\mathbf{t})]\, \partial_{Q_2}\tau_2[Q_{\mathbf{t},2}(\mathbf{t})] + \mathrm{d}_{\tau_2} K_{\mathbf{t},2}(\mathbf{t})\, \partial^3_{Q_2}\tau_2[Q_{\mathbf{t},2}(\mathbf{t})] \\
&= \mathrm{d}^3_{\tau_2} K_{\mathbf{t},2}(\mathbf{t}) \{\partial_{Q_2}\tau_2[Q_{\mathbf{t},2}(\mathbf{t})]\}^3 + 3\, \mathrm{d}^2_{\tau_2} K_{\mathbf{t},2}(\mathbf{t})\, \partial^2_{Q_2}\tau_2[Q_{\mathbf{t},2}(\mathbf{t})]\, \partial_{Q_2}\tau_2[Q_{\mathbf{t},2}(\mathbf{t})] \\
&= \frac{\mathrm{d}^3_{\tau_2} K_{\mathbf{t},2}(\mathbf{t})}{[\mathrm{d}_{\tau_2} Q_{\mathbf{t},2}(\mathbf{t})]^3} + 3 \frac{\mathrm{d}^2_{\tau_2} K_{\mathbf{t},2}(\mathbf{t})}{\mathrm{d}_{\tau_2} Q_{\mathbf{t},2}(\mathbf{t})} \partial^2_{Q_2}\tau_2[Q_{\mathbf{t},2}(\mathbf{t})] \\
&= \frac{\mathrm{d}^3_{\tau_2} K_{\mathbf{t},2}(\mathbf{t})}{[\mathrm{d}_{\tau_2} Q_{\mathbf{t},2}(\mathbf{t})]^3} - 3 \frac{\mathrm{d}^2_{\tau_2} K_{\mathbf{t},2}(\mathbf{t})\, \mathrm{d}^2_{\tau_2} Q_{\mathbf{t},2}(\mathbf{t})}{[\mathrm{d}_{\tau_2} Q_{\mathbf{t},2}(\mathbf{t})]^4}\,.
\end{aligned} \tag{S213c}$$

However, the resultant expressions for Eqs. (S213b) and (S213c) are quite lengthy, so for algebraic simplicity, it is reasonable to approximate them by their values on their respective critical sets – the cusp curve $j_{\mathbf{t}} = 0$ for $\partial^2_{Q_{\mathbf{t},2}} K_{\mathbf{t},2}$ and the focal point $\mathbf{t} = (f, t_2)$ for $\partial^3_{Q_{\mathbf{t},2}} K_{\mathbf{t},2}$. This yields

$$\partial^2_{Q_{\mathbf{t},2}} K_{\mathbf{t},2}(\mathbf{t}) \approx \frac{6f|a|t_2}{\vartheta^3_{\mathbf{t}} |k'_2(t_2)|^3} + O(j_{\mathbf{t}})\,, \quad \partial^3_{Q_{\mathbf{t},2}} K_{\mathbf{t},2}(\mathbf{t}) \approx 6f|a| + O(|\mathbf{t} - \mathbf{t}_f|)\,, \tag{S214}$$

where $\mathbf{t}_f \doteq (f, 0)$ is the coordinate of the focal point. This approximation can be improved (for the same local accuracy) by introducing an additional global constraint, namely, the requirement that the bifurcation set for the saddlepoints of Eq. (S206) be exactly the same as the bifurcation set of the ray system, i.e., the locus of points corresponding to $\Delta[\mathbf{q}(\mathbf{t})] = 0$, where $\Delta(\mathbf{q})$ is defined in Eq. (S170). This yields the approximations

$$\partial^2_{Q_{\mathbf{t},2}} K_{\mathbf{t},2}(\mathbf{t}) \approx 6f|a|t_2 \left| \frac{t_1}{f \vartheta^2_{\mathbf{t}} k'_2(t_2)} \right|^{3/2} i^{3(s_{\mathbf{t}}+1)/2} + O(j_{\mathbf{t}})\,, \quad \partial^3_{Q_{\mathbf{t},2}} K_{\mathbf{t},2}(\mathbf{t}) \approx 6f|a| \left| \frac{t_1}{f \vartheta^2_{\mathbf{t}} k'_2(t_2)} \right|^2 + O(|\mathbf{t} - \mathbf{t}_f|)\,, \tag{S215}$$

where we have defined $s_{\mathbf{t}} \doteq \mathrm{sgn}[k'_2(t_2)]$.

*9. Transforming the inverse MT into standard form*

By combining Eqs. (S206) and (S215), we obtain

$$\Upsilon^\rho_{\mathbf{t}}[\mathbf{q}(\mathbf{t})] = \int_{\mathcal{C}_0} \mathrm{d}\epsilon_\rho \, \exp\left[-i\frac{j_{\mathbf{t}}}{2\vartheta^2_{\mathbf{t}} k'_2(t_2)}\epsilon^2_\rho - if|a|t_2\left|-\frac{f\vartheta^2_{\mathbf{t}} k'_2(t_2)}{t_1}\right|^{-3/2}\epsilon^3_\rho + \frac{i}{4}f|a|\left|\frac{t_1}{f\vartheta^2_{\mathbf{t}} k'_2(t_2)}\right|^2\epsilon^4_\rho\right] , \tag{S216}$$

where $\mathcal{C}_0$ denotes the steepest-descent contour through $\epsilon_\rho = 0$. We shall transform $\Upsilon^\rho_{\mathbf{t}}[\mathbf{q}(\mathbf{t})]$ into the standard Pearcey form [5]. Let

$$\epsilon_\rho = \vartheta_{\mathbf{t}}\left|\frac{2k'_2(t_2)}{t_1}\right|^{1/2}\left|\frac{f}{a}\right|^{1/4} i^{-\frac{s_{\mathbf{t}}+1}{2}}\left(\varepsilon + \frac{t_2}{\sqrt{2}}|fa|^{1/4}\right) , \tag{S217a}$$

$$\mathrm{d}\epsilon_\rho = \vartheta_{\mathbf{t}}\left|\frac{f}{a}\right|^{1/4}\sqrt{\frac{-2k'_2(t_2)}{t_1}}\mathrm{d}\varepsilon \, . \tag{S217b}$$

Then,

$$\Upsilon^\rho_{\mathbf{t}}[\mathbf{q}(\mathbf{t})] = \vartheta_{\mathbf{t}}\left|\frac{f}{a}\right|^{1/4}\sqrt{\frac{-2k'_2(t_2)}{t_1}}\exp\left(i\frac{j_{\mathbf{t}}+f-t_1}{4t_1}ft_2^2\right)\int_{\mathcal{C}_0}\mathrm{d}\varepsilon\,\exp\left(iy_{\mathbf{t}}\varepsilon + ix_{\mathbf{t}}\varepsilon^2 + i\varepsilon^4\right) , \tag{S218}$$

where we have defined

$$x_{\mathbf{t}} \doteq |fa|^{1/2}\,\frac{f-q_1(\mathbf{t})}{|a|q_1(\mathbf{t})} , \quad y_{\mathbf{t}} \doteq \sqrt{2}\,|fa|^{3/4}\,\frac{q_2(\mathbf{t})}{|a|q_1(\mathbf{t})} , \tag{S219}$$

and $\mathcal{C}_0$ is the steepest-descent contour through the saddlepoint $\varepsilon_0 = -t_2|fa|^{1/4}/\sqrt{2}$.

## D. Initial conditions

Far from the caustic, we can evaluate $\Upsilon^\rho_{\mathbf{t}}[\mathbf{q}(\mathbf{t})]$ in the GO limit as

$$\Upsilon^\rho_{\mathbf{t}}[\mathbf{q}(\mathbf{t})] \approx \int_{-\infty}^{\infty}\mathrm{d}\epsilon_\rho\,\exp\left[-i\frac{j_{\mathbf{t}}}{2\vartheta^2_{\mathbf{t}}k'_2(t_2)}\epsilon^2_\rho\right] = \int_{-\infty}^{\infty}\mathrm{d}\epsilon_\rho\,\exp\left\{-\frac{\exp\left[i\,s_{\mathbf{t}}\,\mathrm{sign}(j_{\mathbf{t}})\frac{\pi}{2}\right]}{2}\left|\frac{j_{\mathbf{t}}}{\vartheta^2_{\mathbf{t}}k'_2(t_2)}\right|\epsilon^2_\rho\right\}$$
$$= \vartheta_{\mathbf{t}}\left|\frac{2\pi k'_2(t_2)}{j_{\mathbf{t}}}\right|^{1/2}\exp\left[-i\,s_{\mathbf{t}}\,\mathrm{sign}(j_{\mathbf{t}})\frac{\pi}{4}\right] . \tag{S220}$$

Thus, we can evaluate $\psi_{\mathbf{t}}[\mathbf{q}(\mathbf{t}]$ in the GO limit as

$$\psi_{\mathbf{t}}[\mathbf{q}(\mathbf{t})] = \frac{\sigma_{t_2}\,\alpha_{(0,t_2)}\sqrt{\varphi_{(0,t_2)}}}{\vartheta_{\mathbf{t}}\sqrt{2\pi|k'_2(t_2)|}}\exp\left\{i\chi_{\mathbf{t}} - \frac{i}{2}\beta^\rho_{\mathbf{t}}\left[\mathbf{q}(\mathbf{t})\right] + i\frac{2-s_{\mathbf{t}}}{4}\pi\right\}\vartheta_{\mathbf{t}}\left|\frac{2\pi k'_2(t_2)}{j_{\mathbf{t}}}\right|^{1/2}\exp\left\{-i\,s_{\mathbf{t}}\,\mathrm{sign}(j_{\mathbf{t}})\frac{\pi}{4}\right\}$$
$$= \sigma_{t_2}\,\alpha_{(0,t_2)}\sqrt{\frac{\varphi_{(0,t_2)}}{|j_{\mathbf{t}}|}}\exp\left\{i\chi_{\mathbf{t}} - \frac{i}{2}\beta^\rho_{\mathbf{t}}\left[\mathbf{q}(\mathbf{t})\right] + i\frac{2-s_{\mathbf{t}}-s_{\mathbf{t}}\,\mathrm{sign}(j_{\mathbf{t}})}{4}\pi\right\} . \tag{S221}$$

The assumption $f \gg 1$ implies that the initial surface $(0, q_2)$ lies within the GO regime, while the assumption $\xi < 0$ implies that the ray map $\boldsymbol{\tau}(\mathbf{q})$ is single-valued along the initial surface, and consequently no summation over branches need be performed. Then, since Eq. (S221) evaluates along the initial surface to be

$$\psi_{(0,t_2)}\left[\mathbf{q}(0,t_2)\right] = \sigma_{t_2}\,\alpha_{(0,t_2)}\sqrt{\frac{\varphi_{(0,t_2)}}{f}}\exp\left\{-\frac{i}{2}\beta^\rho_{(0,t_2)}\left[\mathbf{q}(0,t_2)\right] + i\frac{1-s_{\mathbf{t}}}{2}\pi\right\} , \tag{S222}$$

the choice

$$\alpha_{(0,t_2)} = \frac{\sqrt{2\pi}}{\sigma_{t_2}\sqrt{\varphi_{(0,t_2)}}}\exp\left\{\frac{i}{2}\beta^\rho_{(0,t_2)}\left[\mathbf{q}(0,t_2)\right] - \frac{i}{2}ft_2^2 - \frac{ia}{4}ft_2^4 + i\frac{2s_{\mathbf{t}}-1}{4}\pi\right\} \tag{S223}$$

satisfies the initial conditions. Thus, we obtain

$$\psi_{\mathbf{t}}\left[\mathbf{q}(\mathbf{t})\right] = \frac{\Upsilon^{\rho}_{\mathbf{t}}[\mathbf{q}(\mathbf{t})]}{\vartheta_{\mathbf{t}}\sqrt{|k_2'(t_2)|}} \exp\left[ i t_1 + \frac{i}{2} t_1 \left( t_2 + a t_2^3 \right)^2 - \frac{i}{2} f t_2^2 - \frac{ia}{4} f t_2^4 + i \frac{1 + s_{\mathbf{t}}}{4}\pi \right] , \tag{S224}$$

or equivalently,

$$\psi_{\mathbf{t}}\left(\mathbf{q}\right) = \left| \frac{4f}{a q_1^2} \right|^{1/4} \exp\left( i q_1 + i \frac{q_2^2}{2 q_1} \right) \int_{\mathcal{C}_0} \mathrm{d}\varepsilon \, \exp\left( i \left| \frac{4 f^3}{a} \right|^{1/4} \frac{q_2}{q_1} \varepsilon + i \left| \frac{f}{a} \right|^{1/2} \frac{f - q_1}{q_1} \varepsilon^2 + i \varepsilon^4 \right) . \tag{S225}$$

### E. Branch summation

We must now sum Eq. (S225) over all branches of $\mathbf{t} \in \boldsymbol{\tau}(\mathbf{q})$, which, because Eq. (S225) does not have any explicit $\mathbf{t}$ dependence, is equivalent to summing over all real saddlepoints. When $\Delta(\mathbf{q}) \leq 0$, all saddlepoints in Eq. (S225) are real, so

$$\begin{aligned} \psi(\mathbf{q}) &= \sum_{t_2 \in \tau_2(\mathbf{q})} \left| \frac{4f}{a q_1^2} \right|^{1/4} \exp\left( i q_1 + i \frac{q_2^2}{2 q_1} \right) \int_{\mathcal{C}_0(t_2)} \mathrm{d}\varepsilon \, \exp\left( i \left| \frac{4 f^3}{a} \right|^{1/4} \frac{q_2}{q_1} \varepsilon + i \left| \frac{f}{a} \right|^{1/2} \frac{f - q_1}{q_1} \varepsilon^2 + i \varepsilon^4 \right) \\ &= \left| \frac{4f}{a q_1^2} \right|^{1/4} \exp\left( i q_1 + i \frac{q_2^2}{2 q_1} \right) \int_{-\infty}^{\infty} \mathrm{d}\varepsilon \, \exp\left( i \left| \frac{4 f^3}{a} \right|^{1/4} \frac{q_2}{q_1} \varepsilon + i \left| \frac{f}{a} \right|^{1/2} \frac{f - q_1}{q_1} \varepsilon^2 + i \varepsilon^4 \right) . \end{aligned} \tag{S226}$$

When $\Delta(\mathbf{q}) > 0$, only one saddlepoint in Eq. (S225) is real, while the remaining two are complex (and complex conjugate to each other). Let us define

$$\widetilde{\Delta}(\mathbf{q}) \doteq 2 \left( \frac{f - q_1}{|a| q_1} \right)^3 + 27 (5 - \sqrt{27}) \left( \frac{q_2}{|a| q_1} \right)^2 . \tag{S227}$$

As discussed in Refs. [5, 6], only when $\widetilde{\Delta}(\mathbf{q}) > 0$ does

$$\begin{aligned} &\int_{\mathcal{C}_0(t_2)} \mathrm{d}\varepsilon \, \exp\left( i \left| \frac{4 f^3}{a} \right|^{1/4} \frac{q_2}{q_1} \varepsilon + i \left| \frac{f}{a} \right|^{1/2} \frac{f - q_1}{q_1} \varepsilon^2 + i \varepsilon^4 \right) \\ &= \int_{-\infty}^{\infty} \mathrm{d}\varepsilon \, \exp\left( i \left| \frac{4 f^3}{a} \right|^{1/4} \frac{q_2}{q_1} \varepsilon + i \left| \frac{f}{a} \right|^{1/2} \frac{f - q_1}{q_1} \varepsilon^2 + i \varepsilon^4 \right) . \end{aligned} \tag{S228}$$

Otherwise, the integral along the real line also contains the contribution from one of the complex saddlepoints. However, since this contribution is asymptotically subdominant, let us include it for simplicity. (A more careful investigation regarding the role of complex rays in MGO will be investigated in a future publication.) Then, we can perform the summation such that for all $\mathbf{q}$,

$$\psi(\mathbf{q}) = \left| \frac{4f}{a q_1^2} \right|^{1/4} \exp\left( i q_1 + i \frac{q_2^2}{2 q_1} \right) \mathrm{Pe}\left( \left| \frac{f}{a} \right|^{1/2} \frac{f - q_1}{q_1}, \left| \frac{4 f^3}{a} \right|^{1/4} \frac{q_2}{q_1} \right) , \tag{S229}$$

where $\mathrm{Pe}(x, y)$ is the Pearcey function, defined as

$$\mathrm{Pe}(x, y) = \int_{-\infty}^{\infty} \mathrm{d}s \, \exp\left( i s^4 + i x s^2 + i y s \right) . \tag{S230}$$


[1] R. G. Littlejohn, Phys. Rep. **138**, 193 (1986).
[2] R. G. Littlejohn and J. M. Robbins, Phys. Rev. A **36**, 2953 (1987).
[3] N. A. Lopez and I. Y. Dodin, New J. Phys. **22**, 083078 (2020).
[4] H. Kogelnik and T. Li, Appl. Opt. **5**, 1550 (1966).
[5] F. W. J. Olver, D. W. Lozier, R. F. Boisvert, and C. W. Clark, *NIST Handbook of Mathematical Functions* (Cambridge: Cambridge University Press, 2010).
[6] F. J. Wright, J. Phys. A: Math. Gen. **13**, 2913 (1980).
